# Supplementary material for: Finite-Graph-Cover-Based Analysis of Factor Graphs in Classical and Quantum Information Processing Systems
Source: arXiv:2412.05942 source file (2024-12-08)
Supplement: Supplementary file 1 [file SST.tex]

%***************************************************************************
In this appendix, we will use the Gamma function, \textit{i.e.},
$\Gamma(z) \defeq \int_{0}^{\infty} s^{z-1} \e^{-s} \dd{s}$ for $z \in \sC$
with $\Re(z) > 0$. Note that $\Gamma(z) = (z -  1)!$ if $z$ is a
positive-valued integer. However, we will use the Gamma function $ \Gamma $ also with
non-integral real arguments. Moreover, let $S_n$ be the
$(n \! - \! 1)$-dimensional area of the unit sphere in $\sR^n$. It holds that
$S_n = 2 \cdot \pi^{n/2} / \Gamma(n/2)$ (see, \textit{e.g.}, \cite{Folland2001}).

%***************************************************************************

The following lemma contains a useful technical result.

%***************************************************************************

\begin{lemma}
  \label{lemma:special:binomial:sum:1}

  Let $k \in \sZp$. It holds that
  \begin{align*}
    \sum_{\ell=0}^{k}
      \binom{k}{\ell}
        \cdot
        \Gamma(\ell \! + \! 1/2) 
        \cdot 
        \Gamma(k \! - \! \ell \! + \! 1/2)
      &= \frac{S_2}{2}
         \cdot
         k! \ .
  \end{align*}
\end{lemma}

%***************************************************************************

\begin{proof}
  Let $\cvw \defeq (\cw_0, \cw_1)^\tran \in \sR^2$ be the vector with norm one, \textit{i.e.}, $ \cw_0^{2} + \cw_1^{2} = 1 $, as defined in Definition~\ref{sec:SST:def:3}. Using a Fubini-Study measure
  of dimension one, we obtain
  \begin{align*}
    1
      &= \int
           1
         \dd{\muFSsimple(\cvw)} \\
      &\overset{(a)}{=} \int
           \bigl( \cw_0^2 + \cw_1^2 \bigr)^{\! k}
         \dd{\muFSsimple(\cvw)} \\
      &= \int
           \sum_{\ell=0}^{k}
             \binom{k}{\ell}
             \cdot
             \cw_0^{2\ell}
             \cdot
             \cw_1^{2(k-\ell)}
           \dd{\muFSsimple(\cvw)} \\
      &= \sum_{\ell=0}^{k}
           \binom{k}{\ell}
             \cdot
             \int
               \cw_0^{2\ell}
               \cdot
               \cw_1^{2(k-\ell)}
             \dd{\muFSsimple(\cvw)} \\
       &\overset{(b)}{=}  \sum_{\ell=0}^{k}
           \binom{k}{\ell}
           \cdot
           \frac{2 \cdot \Gamma(\ell+1/2) \cdot \Gamma(k-\ell+1/2)}
                {\Gamma(k+1)}
           \cdot
           \frac{1}{S_2},
  \end{align*}
  where step $(a)$ follows from the fact that $\cw_0^2 + \cw_1^2 = 1$
  for all $\cvw = (\cw_0,\cw_1)^\tran$ where the measure $\muFSsimple(\cvw)$
  is nonzero, and where step $(b)$ follows from the main theorem
  in~\cite{Folland2001}.
\end{proof}

%***************************************************************************

We come now to the actual proof of the lemma. By Lemma~\ref{sec:SST:lem:4}, it is equivalent to prove that
\begin{align*}
  \int
    \funcFS_{e,\cpsi_e}\bigl( \vx_{\efi,[M]}, \vx_{\efj,[M]} \bigr)
    \dd{\muFSsimple\bigl( \cvpsi_e \bigr)} 
    &= \begin{cases}
         \frac{1}{|\set{T}_{e,\vt_e}|}
           & \vt_e = \vt_e\bigl(\vx_{\efi,[M]}\bigr) 
            = \vt_e\bigl( \vx_{\efj,[M]} \bigr) 
          \\
         0
           & \text{otherwise}
    \end{cases}
\end{align*}
for all $ \vx_{\efi,[M]}, \vx_{\efj,[M]} \in \set{X}_e^M $.
In the following, we will
use the following notation:
\begin{itemize}

\item We define $d \defeq |\set{
X}_e|$.

\item We assume, without loss of generality, that $\set{X}_e = \{ 0, 1, \ldots, d \! - \! 1 \}$.

\item We write $x$ instead of the more precise $x_e$.

\item We use the short hand $\prod_x$ and $ \sum_{x} $ for $\prod_{x \in \set{X}_e}$ and $ \sum_{x \in \set{X}_e} $, respectively.

\item We let
  $\vk_e = ( k_{e,x} )_{x \in \set{X}_e} = M \cdot \vt_e(\vx_{\efi,[M]})$ and
  $\vk'_e = ( k'_{e,x} )_{x \in \set{X}_e} = M \cdot \vt_e(\vx_{\efj,[M]})$.

\end{itemize}

%***************************************************************************

First, we consider the case where $\vk_e = \vk'_e = \frac{1}{M} \cdot \vt_{e}$. In this case, by the definition of $ \funcFS_{e,\cpsi_{e}} $ in Definition~\ref{sec:SST:def:3}, we have
%-----------------------------------------------------------------------
\begin{align*}
    \int
        \funcFS_{e,\cpsi_e}(x_{\efi}, x_{\efj})
    \dd{\muFSsimple(\cvpsi_{e})}
    &=  
    |\set{B}_{\set{X}_e^M}| \cdot
    \int
        \prod_{x}
           |\cpsi_e(x)|^{2k_{e,x}}
    \dd{\muFSsimple(\cvpsi_{e})}.
\end{align*}
%-----------------------------------------------------------------------
Using a Fubini-Study
measure of dimension $|\set{X}_e|$, we get
\begin{align*}
    \hspace{0.5 cm}&\hspace{-0.5 cm}\int
        \prod_{x}
        |\cpsi_e(x)|^{2k_{e,x}}
       \dd{\muFSsimple(\cvpsi_{e})} 
     \nonumber\\
    &= \int
         \prod_x
           \bigl( \cw_{x,0}^2 + \cw_{x,1}^2 \bigr)^{\! k_{e,x}}
       \dd{\muFSsimple(\cvw)} \nonumber \\
    &= \int
         \prod_x
           \sum_{\ell_{e,x}=0}^{k_{e,x}}
             \binom{k_{e,x}}{\ell_{e,x}}
             \cdot \cw_{x,0}^{2\ell_{e,x}}
             \cdot
             \cw_{x,1}^{2(k_{e,x}-\ell_{e,x})}
       \dd{\muFSsimple(\cvw)} \nonumber \\
    &= \sum_{\ell_{e,0}=0}^{t_{e,0}}
       \cdots
       \sum_{\ell_{e,d-1}=0}^{t_{e,d-1}}
         \left(
           \prod_x
             \binom{k_{e,x}}{\ell_{e,x}}
         \right)
         \cdot
         \int
           \prod_x
             \cw_{x,0}^{2\ell_{e,x}}
             \cdot
             \cw_{x,1}^{2(k_{e,x}-\ell_{e,x})}
           \dd{\muFSsimple(\cvw)} \nonumber  \\
    &\overset{(a)}{=} \sum_{\ell_{e,0}=0}^{t_{e,0}}
       \cdots
       \sum_{\ell_{e,d-1}=0}^{t_{e,d-1}}
         \left(
           \prod_x
             \binom{k_{e,x}}{\ell_{e,x}}
         \right)
         \cdot
           \frac{2 
                   \cdot
                   \Bigl(
                     \prod_x
                       \Gamma(\ell_{e,x}+1/2) 
                       \cdot 
                       \Gamma(k_{e,x}-\ell_{e,x}+1/2)
                   \Bigr)
                 }
                 {\Gamma(M + d) \cdot S_{2d}}
       \nonumber \\
    &= \frac{2}{S_{2d}}
       \cdot
       \frac{1}{(M+d-1)!}
       \cdot
       \prod_x
         \sum_{\ell_{e,x}=0}^{k_{e,x}}
           \binom{k_{e,x}}{\ell_{e,x}}
           \cdot
           \Gamma(\ell_{e,x}+1/2) 
           \cdot 
           \Gamma(k_{e,x}-\ell_{e,x}+1/2) \nonumber \\
    &\overset{(b)}{=} \frac{S_2^d}{2^{d-1} \cdot S_{2d}}
       \cdot
       \frac{\prod_x (k_{e,x}!)}{(M+d-1)!} \nonumber \\
    &\overset{(c)}{=} (d \! - \! 1)!
       \cdot
       \frac{\prod_x (k_{e,x}!)}{(M+d-1)!} \nonumber \\
    &= \frac{1}{\binom{d+M-1}{M}}
       \cdot
       \frac{1}{ \binom{M}{k_0, \ldots, k_{d-1}} } \nonumber \\
    &\overset{(d)}{=} \frac{1}{|\set{B}_{\set{X}_e^M}|}
       \cdot
       \frac{1}{|\set{T}_{e,\vt_e}|}, 
\end{align*}
where step $(a)$ follows from the main theorem in~\cite{Folland2001} and
$\sum_x k_{e,x} = M$, where step $(b)$ follows from
Lemma~\ref{lemma:special:binomial:sum:1}, where step $(c)$ follows
from $S_2 = 2 \pi$ and $S_{2d} = 2 (\pi^d) / \Gamma(d) = 2 (\pi^d) / (d-1)!$, and where step $(d)$ follows from Lemma~\ref{sec:SST:lem:2}.

%***************************************************************************

Let us now consider the case $\vk_e \neq \vk'_e$, \ie, $ \vt_e\bigl(\vx_{\efi,[M]}\bigr) \neq \vt_e\bigl( \vx_{\efj,[M]} \bigr) $. In this case there is at
least one $x \in \set{X}_e$ such that $k_{e,x} \neq k'_{e,x}$. (In fact, there
must be at least two $x \in \set{X}_e$ such that $k_{e,x} \neq k'_{e,x}$ because
$\sum_x k_{e,x} = \sum_x k'_{e,x} = M$.) Let $\alpha_x \in \sR$,
$x \in \set{X}_e$, be some parameters. Using a Fubini-Study measure of dimension
$|\set{X}_e|$, we consider the expressions
\begin{align}
  \int
    \left(
      \prod_x
        \cpsi_e(x)^{k_{e,x}}
    \right)
    \cdot
    \left(
      \prod_x
        \Bigl( \overline{\cpsi_e(x)} \Bigr)^{\! k'_{e,x}}
    \right)
  \dd{\muFSsimple(\cvpsi)},
    \label{sec:SST:eqn:6} \\
  \int
    \left(
      \prod_x
        \left(
          \e^{\imagunit \alpha_k} \cdot \cpsi_e(x)
        \right)^{k_{e,x}}
    \right)
    \cdot
    \left(
      \prod_x
        \left(
          \overline{\e^{\imagunit \alpha_k} \cdot \cpsi_e(x)}
        \right)^{\! k'_{e,x}}
    \right)
  \dd{\muFSsimple(\cvpsi)}.
      \label{sec:SST:eqn:4}
\end{align}
Because of symmetries of the measure
$\muFSsimple$, the expressions in~\eqref{sec:SST:eqn:6}
and~\eqref{sec:SST:eqn:4} must give the same numerical
value. However, the expression in~\eqref{sec:SST:eqn:4} is
equal to
\begin{align}
  \e^{\imagunit \sum_x \alpha_x \cdot (k_{e,x} - k'_{e,x})}
  \cdot
  \int
    \left(
      \prod_x
        \bigl( \cpsi_e(x) \bigr)^{k_{e,x}}
    \right)
    \cdot
    \left(
      \prod_x
        \Bigl( \overline{\cpsi_e(x)} \Bigr)^{\!\! k'_{e,x}}
    \right)
  \dd{\muFSsimple(\cvpsi)}.
      \label{sec:SST:eqn:5}
\end{align}
Because of the assumptions on $\vk_e$ and $\vk'_e$, it is easy to find
$\alpha_x \in \sR$, $x \in \set{X}_e$, such that
$\e^{\imagunit \sum_x \alpha_x \cdot (k_{e,x} - k'_{e,x})} \neq 1$. Given this, the
only possibility for all expressions
in~\eqref{sec:SST:eqn:6}--\eqref{sec:SST:eqn:5}
to be the same is that they are all equal to zero. From this observation one
can conclude that
\begin{align*}
    \int
    \funcFS_{e,\cpsi_e}(\vx_{e,f}, \vx_{e,f'})
    \dd{\muFSsimple(\cvpsi)}
    &= |\set{B}_{\set{X}_e^M}| \cdot
    \int
         \left(
           \prod_x
             \bigl( \cpsi_e(x) \bigr)^{\! k_{e,x}}
         \right)
         \cdot
         \left(
           \prod_x
             \Bigl( \overline{\cpsi_e(x)} \Bigr)^{\!\! k'_{e,x}}
         \right)
       \dd{\muFSsimple(\cvpsi)}
       \nonumber\\
    & = 0.
\end{align*}

%***************************************************************************
%***************************************************************************

\ifx\sectionheaderonnewpage\x
\clearpage
\fi
