# Supplementary material for: Finite-Graph-Cover-Based Analysis of Factor Graphs in Classical and Quantum Information Processing Systems
Source: arXiv:2412.05942 source file (2024-12-08)
Supplement: Supplementary file 2 [file check_cond_lower.tex]

\begin{figure}
    \centering
    \captionsetup{font=scriptsize}
    \begin{adjustbox}{minipage=\linewidth,scale=0.98}
    \subfloat[\label{sec:CheckCon:fig:8:subfig:1}]{
    \begin{minipage}[t]{0.45\linewidth}
      \centering
      \begin{tikzpicture}[on grid, auto, scale=0.98]
        \input{figures/lct_examples/scale_small.tex}
        \input{figures/head_files_figs.tex}
        \input{figures/lct_examples/penfg/background_nodes_original.tex}
        \node[state_long] (f1) at (-\ldis,0) [label=above: $\LCT{f}_{i}$] {};
        \node[state_long] (f2) at (\ldis,0) [label=above: $\LCT{f}_{j}$] {};
        % draw the lines
        \input{figures/lct_examples/penfg/background_lines_orignal.tex}
        %----------------------------------------------------------------------
        \begin{pgfonlayer}{main} 
            \node (x1) at (0,-0.2*\sdis) 
            [label=above: $\vx_{\pone}$] {}; 
            \node (x3) at (-1.5*\ldis,1.5*\sdis) 
            [label=above: $\LCTv{x}_{\ptwo}$] {}; 
            \node (x4) at (-1.5*\ldis,-1.5*\sdis) 
            [label=below: $\LCTv{x}_{\pthre}$] {};

            \node (x3) at (1.5*\ldis,1.5*\sdis) 
            [label=above: $\LCTv{x}_{\pfor}$] {}; 
            \node (x4) at (1.5*\ldis,-1.5*\sdis) 
            [label=below: $\LCTv{x}_{\pfif}$] {}; 
        \end{pgfonlayer}
        %----------------------------------------------------------------------
      \end{tikzpicture}
    \end{minipage}
  }
  \subfloat[\label{sec:CheckCon:fig:8:subfig:2}]{
    \begin{minipage}[t]{0.45\linewidth}
      \centering
      \begin{tikzpicture}[on grid, auto, scale=0.98]
        \input{figures/lct_examples/scale_small.tex}
        \input{figures/head_files_figs.tex}

        \input{figures/proof_lower_bound/background_nodes_after_lct_proof_s.tex}
        \input{figures/proof_lower_bound/background_variables_evd_s.tex}
        
        \input{figures/lct_examples/penfg/variables_after_lct_clb.tex}

        \input{figures/lct_examples/penfg/background_lines.tex}
        \input{figures/lct_examples/penfg/otb_dashed_boxes_evd_after_lct.tex}
        
      \end{tikzpicture}
    \end{minipage}
  }

  \subfloat[\label{sec:CheckCon:fig:8:subfig:3}]{
    \begin{minipage}[t]{0.45\linewidth}
      \centering
      \begin{tikzpicture}[on grid, auto, scale=0.98]
        \input{figures/proof_lower_bound/scale_large_pesnfg_lower_bound.tex}
        \input{figures/head_files_figs.tex}
        \tikzstyle{state_dash5}=[shape=rectangle, draw, dashed, minimum width= 1.7*\sdis cm, minimum height = 4.1*\ldis cm,outer sep=-0.3pt, fill=black!10]

        \input{figures/proof_lower_bound/background_nodes_after_lct_proof.tex}
        \input{figures/proof_lower_bound/function_otb_lct.tex}
        \input{figures/proof_lower_bound/background_variables_EVD_l}

        \input{figures/lct_examples/penfg/variables_after_lct_clb.tex}
        \input{figures/lct_examples/penfg/background_lines.tex}
        \input{figures/lct_examples/penfg/otb_dashed_boxes_evd_after_lct.tex}
  
      \end{tikzpicture}
    \end{minipage}
  }
  \subfloat[\label{sec:CheckCon:fig:8:subfig:4}]{
    \begin{minipage}[t]{0.45\linewidth}
      \centering
      \begin{tikzpicture}[on grid, auto, scale=0.98]
        \input{figures/proof_lower_bound/scale_large_pesnfg_lower_bound.tex}
        \input{figures/head_files_figs.tex}
        \begin{pgfonlayer}{behind} 
            \node[state_dash7] (db1) at (-0.8*\ldis,-0.6*\sdis) 
            [label=above: $ \MLUfn{i} $] {};
            \node[state_dash7] (db2) at (0.8*\ldis,-0.6*\sdis)  [label=above: 
            $ \MLUfn{j} $] {};

            \node[state_dash7] (db1) at (-0.8*\ldis,-5.18*\sdis) 
            [label=below: $ \overline{\MLUfn{i}} $] {};
            \node[state_dash7] (db2) at (0.8*\ldis,-5.18*\sdis)  
            [label=below: $ \overline{\MLUfn{j}} $] {};
        \end{pgfonlayer}

        \input{figures/proof_lower_bound/background_nodes_after_lct_proof.tex}
        \input{figures/proof_lower_bound/background_variables_EVD_l0.tex}
        \input{figures/proof_lower_bound/function_otb_lct.tex}
        
        \input{figures/lct_examples/penfg/variables_after_lct_clb.tex}
        \input{figures/lct_examples/penfg/background_lines.tex}
      \end{tikzpicture}
    \end{minipage}
  }
  \end{adjustbox}
  \caption{Illustrating the main idea of the proof in Appendix~\ref{apx:check_cond_lower} by an example PE-NFG.}
\end{figure}

To outline the main idea of the proof,  we introduce the following definitions for each $f \in \setF$.
%----------------------------------------------------------------------------
\begin{definition}
    We consider the Cholesky decomposition of the Choi-matrix representation $ \matr{C}_{\LCT{f}} $ provided in Item~\ref{prop:DENFG:LCT:1:item:5} in Proposition~\ref{prop:DENFG:LCT:1}, which yields the function $ \LCT{L}_{f} $ and the set $ \LCTset{L}_{f} $. Without loss of generality, we suppose that $ \setpf = (1,\ldots,|\setpf|) $.
    %----------------------------------------------------------------------------
    \begin{enumerate}
      \item We define 
        \begin{align*}
            \LCTv{U}_{L,f} \defeq 
            \Bigl( 
                \LCT{U}_{L,f} \bigl( \LCTellf', \LCTellf \bigr)
            \Bigr)_{ \LCTellf', \LCTellf \in \LCTset{L}_{f} } 
        \end{align*} 
        to be a unitary matrix with row indices $ \LCTellf' $ and column indices $ \LCTellf $ such that
        \begin{align*}
            \sum_{\LCTellf \in \LCTset{L}_{f}} 
            \LCT{U}_{L,f} \bigl( \LCTellf', \LCTellf \bigr)
            \cdot  
            \overline{ \LCT{U}_{L,f} \bigl( \LCTellf'', \LCTellf \bigr) }
            &= \Bigl[ \LCTellf' \! = \! \LCTellf'' \Bigr], \qquad 
            \LCTellf', \LCTellf'' \in \LCTset{L}_{f}, \nonumber\\
            \LCTv{U}_{L,f}(\LCTellf,0) &= 
            \frac{1}{ \sqrt{\LCT{f}(\bm{0})}  }
            \cdot
            \overline{ \LCT{L}_{f}(\bm{0},\LCTellf) }, \qquad 
            \LCTellf \in \LCTset{L}_{f}.
      \end{align*}
      %------------------------------------------------------------------------
      % which implies
      % %-----------------------------------------------------------------------
      % \begin{align*}
      %   \bigl( \LCTv{U}_{L,f}( :, 0 ) \bigr)^{\Herm}
      %   \cdot \LCTv{U}_{L,f}( :, 0 )
      %   = 1.
      % \end{align*}
      % %-----------------------------------------------------------------------

        \item We define $ \LCTv{L}_{f} $ as follows:
        \begin{align}
            \LCTv{L}_{f} \defeq 
            \biggl( 
              \LCT{L}_{f}\Bigl( \LCTv{x}_{\setpf},\LCTell{f} \Bigr) 
            \biggr)_{ \LCTv{x}_{\setpf} \in \LCTset{X}_{\setpf}, 
            \LCTell{f} \in \LCTset{L}_{f} }.
            \label{eqn: def of matrix Lf}
        \end{align}
        This matrix has row indices $ \LCTv{x}_{\setpf} = ( \LCT{x}_{1},\ldots,\LCT{x}_{|\setpf|} ) $, which take values from $ (0,\ldots,0) $, $ (1,\ldots,0) $ to $ ( \bigl| \LCTsetx_{1} \bigr|-1,\ldots, \bigl| \LCTsetx_{|\setpf|} \bigr|-1) $, and column indices $ \LCTell{f_{i}} $, which take values from $ 0 $, $ 1 $ to $ |\LCTset{L}_{f}|-1 $.
        Note that 
        $ \bigl| \LCTset{L}_{f} \bigr| = \bigl| \LCTsetx_{\setpf} \bigr| $.
        % and $ \bm{0} $ is the all-zero vector of size $|\setpf|$.

        \item We define $ \mMLUf $ to be a matrix having the same row and column indexing as $\LCTv{L}_{f}$:
        %------------------------------------------------------------------------
        \begin{align*}
            \mMLUf \defeq
            \Bigl( \MLUf\bigl( \LCTv{x}_{\setpf}, \LCTellf \bigr) 
            \Bigr)_{ \LCTv{x}_{\setpf} \in \LCTset{X}_{\setpf}, \LCTellf \in \LCTset{L}_{f} },
        \end{align*}
        %------------------------------------------------------------------------
        where the entries are defined to be
        \begin{align*}
            \MLUf\bigl( \LCTv{x}_{\setpf}, \LCTellf \bigr) 
            \defeq 
            \sum_{\LCTellf' \in \LCTset{L}_{f}}
            \LCT{L}_{f}\Bigl( \LCTv{x}_{\setpf},\LCTellf' \Bigr)
            \cdot \LCT{U}_{L,f} \bigl( \LCTellf', \LCTellf \bigr).
        \end{align*}  
        By the Cholesky decomposition in~\eqref{sec:LCT:eqn:17}, the matrix $ \mMLUf $ satisfies the following property:
        %------------------------------------------------------------------------
        \begin{align}
            \mMLUf(:,0) = \LCTv{L}_{f} \cdot \LCTv{U}_{L,f}(:,0)
            = \frac{1}{ \sqrt{\LCT{f}(\bm{0})} } 
            \cdot 
            \LCTv{L}_{f} 
            \cdot \LCTv{L}_{f}( \bm{0},: )^{\Herm}
            &= \frac{1}{ \sqrt{\LCT{f}(\bm{0})} } 
            \cdot \matr{C}_{\LCT{f}}( :, \bm{0} ), \label{sec:CheckCon:eqn:39}
        \end{align}
        %------------------------------------------------------------------------
        % where $ \matr{C}_{\LCT{f}} $ is . 
        % Following the similar idea in the proof of Lemma~\ref{lem: nonnegative of ZBSPA for PE-NFG}, we know that $ \LCT{f}(\bm{0}) = Z_{\LCT{f}}( \LCTv{\mu} ) \in \sR_{\geq 0} $ for the SPA fixed-point message vector $ \LCTv{\mu} $ for $ \LCT{\sfN} $.

        \item For $ M \in \sZpp $, we define the collection of variables $ \LCTv{\ell}^{(M)} $ to be
        %-----------------------------------------------------------------------
        \begin{align*}
            \LCTv{\ell}^{(M)} \defeq 
            \bigl( \LCT{\ell}_{f,m} \bigr)_{f \in \setF, m \in [M]}
            \in \prod_{f} \LCTset{L}_{f}^{M}.
            % \qquad 
            % \ell'^{(M)} \defeq ( \ellfm' )_{f \in \setF, m \in [M]}
            % \in \prod_{f} \set{L}_{f}^{M}, \qquad 
            % \ell''^{(M)} \defeq ( \ellfm'' )_{f \in \setF, m \in [M]}
            % \in \prod_{f} \set{L}_{f}^{M},
        \end{align*}
        %-----------------------------------------------------------------------
        To simplify notation, if there is no ambiguity, 
        we use $ \sum_{ \LCT{\ell}_{f} } $ for each $ f \in \setF $ and $ \sum_{\LCTv{\ell}^{(M)}} $ 
        instead of 
        $ \sum_{ \LCT{\ell}_{f} \in \LCTset{L}_{f} } $ 
        for each $ f \in \setF $ and
        $ \sum_{ \LCTv{\ell}^{(M)} \in \prod_{f} \LCTset{L}_{f}^{M} } $, respectively.

        \item We define the vectors $ \cvpsi_{\setpf,f} $ and $ \cvpsi_{\upsetpf,f} $ to be
        \begin{align*}
            \cvpsi_{\setpf,f}
            \defeq
            \bigotimes_{e \in \setpf} 
            \cvpsi_{e,f} \in 
            \sC^{\prod_{e \in \setpf}|\LCTset{X}_{e}|},
            \qquad
            \cvpsi_{\upsetpf,f}
            \defeq
            \bigotimes_{\upe \in \upsetpf} 
            \cvpsi_{\upe,f} \in 
            \sC^{\prod_{\upe \in \upsetpf}|\LCTset{X}_{\upe}|}
        \end{align*}
    \end{enumerate}
    \edefinition
\end{definition}

The proof started by considering a
specific PE-NFG $\LCT{\graphN}$ and assume that a part of it looks as shown in Fig.~\ref{sec:CheckCon:fig:8:subfig:1}. The proof then proceeds through the following steps.
%----------------------------------------------------------------------------
\begin{enumerate}
    \item The Choi-matrix representations of $ \LCT{f}_{i} $ and $ \LCT{f}_{j} $, denoted as $ \matr{C}_{\LCT{f}_{i}} $ and $ \matr{C}_{\LCT{f}_{j}} $, respectively, are PSD matrices. The PE-NFG in Fig.~\ref{sec:CheckCon:fig:8:subfig:2} is obtained from the PE-NFG
    in Fig.~\ref{sec:CheckCon:fig:8:subfig:1} by applying the Cholesky decomposition in~\eqref{sec:LCT:eqn:17} to $ \matr{C}_{\LCT{f}_{i}} $ and $ \matr{C}_{\LCT{f}_{j}} $.

    \item The PE-NFG in Fig.~\ref{sec:CheckCon:fig:8:subfig:3} is obtained from the PE-NFG
    in Fig.~\ref{sec:CheckCon:fig:8:subfig:2} by introducing suitable opening-the-box operations. Since $ \LCTv{U}_{L,f} $ is a unitary matrix for all $ f \in \setF $,
    the partition function of the PE-NFG in Fig.~\ref{sec:CheckCon:fig:8:subfig:3} is equal to that of the PE-NFG
    in Fig.~\ref{sec:CheckCon:fig:8:subfig:2}.

    \item The PE-NFG in Fig.~\ref{sec:CheckCon:fig:8:subfig:4} is obtained from the PE-NFG
    in Fig.~\ref{sec:CheckCon:fig:8:subfig:3} by applying suitable closing-the-box operations and setting $ \LCTell{f_{i}} = \LCTell{f_{j}} = 0  $. 
    For example, the exterior function of the upper left dashed box in Fig.~\ref{sec:CheckCon:fig:8:subfig:4} is given by
    %------------------------------------------------------------------------
    \begin{align*}
        \MLUfn{i}(\LCTv{x}_{\setpfi},0) &= 
        \sum_{\LCTell{f_{i}}'}
        \LCT{L}_{f_{i}}\Bigl( \LCTv{x}_{\setpfi},\LCTell{f_{i}}' \Bigr)
        \cdot \LCT{U}_{L,f_{i}} \bigl( \LCTell{f_{i}}', 0 \bigr)
        = \frac{1}{\sqrt{\LCT{f}_{i}(\bm{0})}}
        \cdot C_{\LCT{f}_{i}}( \LCTv{x}_{\setpfi}, \bm{0} ), \qquad 
        \LCTv{x}_{\setpfi} \in \LCTset{X}_{\setpfi}.
    \end{align*}
    %------------------------------------------------------------------------

    \item Finally, it is shown that the partition function of the PE-NFG in Fig.~\ref{sec:CheckCon:fig:8:subfig:4} is smaller than or equal to that of the PE-NFG in Fig.~\ref{sec:CheckCon:fig:8:subfig:3}. The details of this step are provided in the remaining part of this appendix.
\end{enumerate}
%----------------------------------------------------------------------------
These steps outline the main idea of the proof and describe how the PE-NFG evolves through various transformations to establish the desired result.

%----------------------------------------------------------------------------
\begin{lemma} \label{sec:CheckCon:lem:integral w.r.t. psi dot e equals psi e}
    It holds that
    %------------------------------------------------------------------------
    \begin{align*}
        &\int
            \prod_{m}
            \prod_f 
            \cvpsi_{\upsetpf,f}
            \cdot \overline{ \mMLUf\bigl( :, \LCTell{f,m} \bigr) }
        \prod_{\upe \in \upsetEfull}
        \dd{\muFSsimple(\cvpsi_{\upe})}
        = \overline{ \int
            \prod_{m}
            \prod_f 
            \cvpsi_{\setpf,f}
            \cdot \mMLUf\bigl( :, \LCTell{f,m} \bigr)
        \prod_{e \in \setEfull}
        \dd{\muFSsimple\bigl( \cvpsi_{e} \bigr)} 
        }, \qquad 
        \LCTv{\ell}^{(M)} 
        \in \prod_{f} \LCTset{L}_{f}^{M}.
    \end{align*}
    %------------------------------------------------------------------------
\end{lemma}
%----------------------------------------------------------------------------
%----------------------------------------------------------------------------
\begin{proof}
    The proof is similar to the derivations of the equalities in~\eqref{sec:SST:eqn:34} in Appendix~\ref{apx:property of ZBM for PENFG}, and thus the details are omitted here. 
\end{proof}
%----------------------------------------------------------------------------
We obtain
%----------------------------------------------------------------------------
\begin{align}
    \hspace{0.25cm}&\hspace{-0.25cm}\Biggl(
            \prod_{e \in \setEfull}
            |\set{B}_{\LCTsetx_{e}^M}|^{2}
    \Biggr)^{\!\! -1}\cdot
    \bigl( \ZBM(\graphN) \bigr)^{\! M}
    \nonumber\\
    % &\overset{(a)}{=}
    % \Biggl(
    %         \prod_{e \in \setEfull}
    %         |\set{B}_{\LCTsetx_{e}^M}|^{2}
    % \Biggr)^{-1}\cdot
    % \int \ZSSTM(\LCTavgalt{\graphN},\cvpsiavgalt) 
    % \dd{\muFSsimple\bigl( \cvpsiavgalt \bigr)}
    % \nonumber\\
    &\overset{(a)}{=}
    % \Biggl(
    %     \prod_{e \in \setEfull}
    %     |\set{B}_{\LCTsetx_{e}^M}|^{2}
    % \Biggr)
    % \cdot
    \int
        \prod_f 
          \Bigl( 
            \ZSSTLCTf\bigl( \cvpsi_{\psetpf} \bigr) 
          \Bigr)^{\!\! M}
    \dd{\muFSsimple\bigl( \cvpsiavgalt \bigr)}
    \nonumber
    \\
    &\overset{(b)}{=}
    % \Biggl(
    %     \prod_{e \in \setEfull}
    %     |\set{B}_{\LCTsetx_{e}^M}|^{2}
    % \Biggr)
    % \cdot
    \int
        \prod_f \left(
          \sum_{\LCTellf}
          \left( 
            \sum_{\LCTv{x}_{\setpf}}
            \LCT{L}_{f}\bigl( \LCTv{x}_{\setpf},\LCTellf \bigr) 
            \cdot
            \prod_{e \in \setpf} 
            \cpsi_{e,f}(\LCT{x}_{e}) 
          \right)
        \cdot
        \left( 
            \sum_{\LCTv{x}_{\upsetpf}}
            \overline{ \LCT{L}_{f}\bigl( \LCTv{x}_{\upsetpf},\LCTellf \bigr) }
            \cdot
            \prod_{\upe \in \upsetpf} 
            \cpsi_{\upe,f}(\LCT{x}_{\upe}) 
      \right)
    \right)^{\!\!\!\! M}
    \dd{\muFSsimple\bigl( \cvpsiavgalt \bigr)}
    \nonumber \\
    &\overset{(c)}{=}
    \int
        \prod_f \biggr(
            \cvpsi_{\setpf,f}^{\tran}
            \cdot 
            \LCTv{L}_{f}
            % \right)
            \cdot 
            % \Bigl( 
            \LCTv{L}_{f}^{\Herm}
            \cdot 
            \cvpsi_{\upsetpf,f}
            % \Bigr)^{\!\! \Herm}
        \biggl)^{\!\! M}
    \dd{\muFSsimple\bigl( \cvpsiavgalt \bigr)}
    \nonumber \\
    &\overset{(d)}{=}
    \int
        \prod_f \biggr(
                \cvpsi_{\setpf,f}^{\tran}
                \cdot 
                \mMLUf
            % \right)
                \cdot 
                \mMLUf^{\Herm}
                \cdot
                \cvpsi_{\upsetpf,f}
        \biggl)^{\!\! M}
    \dd{\muFSsimple\bigl( \cvpsiavgalt \bigr)}
    \nonumber \\
    &=
    \sum_{\LCTv{\ell}^{(M)}}
    \int
        \prod_{m}
        \prod_f 
        % \left(
            % \left(
                \cvpsi_{\setpf,f}^{\tran}
                \cdot 
                \mMLUf\bigl( :, \LCTell{f,m} \bigr)
            % \right)
            \cdot 
            % \left( 
                \cvpsi_{\upsetpf,f}^{\tran}
                \cdot \overline{ \mMLUf\bigl( :, \LCTell{f,m} \bigr) }
            % \right)
        % \right)
    \dd{\muFSsimple\bigl( \cvpsiavgalt \bigr)}
    \nonumber \\
    &\overset{(e)}{=}
    \sum_{\LCTv{\ell}^{(M)}}
    \int
        \prod_{m}
        \prod_f 
        % \Biggl(
            \cvpsi_{\setpf,f}^{\tran}
            \cdot 
            \mMLUf\bigl( :, \LCTell{f,m} \bigr)
        % \Biggr)
    \prod_{e \in \setEfull}
    \dd{\muFSsimple\bigl( \cvpsi_{e} \bigr)}
    \cdot 
        \int
            \prod_{m}
            \prod_f 
            % \left(
                \cvpsi_{\upsetpf,f}^{\tran}
                \cdot \overline{ \mMLUf\bigl( :, \LCTell{f,m} \bigr) }
            % \right)
        \prod_{\upe \in \upsetEfull}
        \dd{\muFSsimple(\cvpsi_{\upe})}
    \nonumber \\
    &\overset{(f)}{=}
    \sum_{\LCTv{\ell}^{(M)}}
    \Biggl| \int
        \prod_{m}
        \prod_f 
        % \Biggl(
            \cvpsi_{\setpf,f}^{\tran}
            \cdot 
            \mMLUf\bigl( :, \LCTell{f,m} \bigr)
        % \Biggr)
    \prod_{e \in \setEfull}
    \dd{\muFSsimple\bigl( \cvpsi_{e} \bigr)} \Biggr|^{2}
    \nonumber \\
    &\geq 
    \sum_{\LCTv{\ell}^{(M)}}
    \Bigl[ \LCTell{f,m} = 0,\, \forall f \in \setF,\, m \in [M] \Bigr]
    \cdot \Biggl| \int
        \prod_{m}
        \prod_f 
        % \Biggl(
            \cvpsi_{\setpf,f}^{\tran}
            \cdot 
            \mMLUf\bigl( :, \LCTell{f,m} \bigr)
        % \Biggr)
    \prod_{e \in \setEfull}
    \dd{\muFSsimple\bigl( \cvpsi_{e} \bigr)} \Biggr|^{2}
    \nonumber\\
    &=
    \Biggl| \int
        \prod_f 
        \Bigl(
           \cvpsi_{\setpf,f}^{\tran}
            \cdot 
            \mMLUf( :, 0 )
        \Bigr)^{\!\! M}
    \prod_{e \in \setEfull}
    \dd{\muFSsimple\bigl( \cvpsi_{e} \bigr)} \Biggr|^{2}
    \nonumber \\
    &\overset{(g)}{=}
    \bigl( \ZBSPA(\graphN) \bigr)^{\!-M}
    \cdot \Biggl| \int 
    \prod_f
    \Bigl( 
        \cvpsi_{\setpf,f}^{\tran}
        \cdot 
        \matr{C}_{\LCT{f}}(:,\bm{0})
    \Bigr)^{\!\! M}
    \prod_{e \in \setEfull}
    \dd{\muFSsimple\bigl( \cvpsi_{e} \bigr)}
    \Biggr|^{2},
    \nonumber\\
    &\overset{(h)}{=}
    \bigl( \ZBSPA(\graphN) \bigr)^{\! -M}
    \cdot \Biggl| \int 
    \prod_f
    \Biggl( 
        \sum_{\LCTv{x}_{\setpf}}
        \LCT{f}( \LCTv{x}_{\setpf}, \bm{0} )
        \prod_{e \in \setpf} 
        \cpsi_{e,f}(\LCT{x}_{e}) 
    \Biggr)^{\!\!\! M}
    \prod_{e \in \setEfull}
    \dd{\muFSsimple(\cvpsi_{e})}
    \Biggr|^{2},
    % \nonumber \\
    % &=
    % \frac{1}{ \bigl( \ZBSPA(\graphN) \bigr)^{M} } 
    % \cdot \Biggl| \int 
    % \prod_f
    % \Bigl( 
    %     \bigotimes_{e \in \setpf} 
    %     \cvpsi_{e,f}^{\tran}
    %     \cdot 
    %     \matr{C}_{\LCT{f}}(:,\bm{0})
    % \Bigr)^{M}
    % \prod_{e \in \setEfull}
    % \dd{\muFSsimple\bigl( \cvpsi_{e} \bigr)}
    % \Biggr|^{2}, \label{sec:CheckCon:eqn:Zsst M-th power ineq}
\end{align}
%----------------------------------------------------------------------------
%----------------------------------------------------------------------------
\begin{itemize}
    \item where step $(a)$ follows from the expression of $ \ZBM $ in~\eqref{sec:CheckCon:eqn:42},

    \item where step $(b)$ follows from the definition of $ \ZSSTLCTf $ in~\eqref{sec:algsin:eqn:158} and the decomposition of $ \LCT{f} $ 
    in~\eqref{sec:LCT:eqn:17},

    \item where step $(c)$ follows from definition of $ \LCTv{L}_{f} $ in~\eqref{eqn: def of matrix Lf},

    \item where step $(d)$ follows from the fact that $ \LCTv{U}_{L,f} $ is a unitary matrix, \ie,
    %----------------------------------------------------------------------------
    \begin{align*}
        \mMLUf \cdot \mMLUf^{\Herm}
        = \LCTv{L}_{f} \cdot \LCTv{U}_{L,f}
        \cdot \LCTv{U}_{L,f}^{\Herm} \cdot \LCTv{L}_{f}^{\Herm}
        = \LCTv{L}_{f} \cdot \LCTv{L}_{f}^{\Herm},
    \end{align*}
    %----------------------------------------------------------------------------

    \item where step $(e)$ follows from
    \begin{align*}
        \dd{\muFSsimple\bigl( \cvpsiavgalt \bigr)} =
        \Biggl( \prod_{e \in \setEfull} 
            \dd{\muFSsimple\bigl( \cvpsi_{e} \bigr)} 
        \Biggr)
        \cdot
        \Biggl( \prod_{\upe \in \upsetEfull} 
            \dd{\muFSsimple\bigl( \cvpsi_{\upe} \bigr)} 
        \Biggr), \qquad 
        \int \dd{\muFSsimple\bigl( \cvpsi_{e} \bigr)}  
        = \int \dd{\muFSsimple\bigl( \cvpsi_{\upe} \bigr)} = 1, \qquad
        \pe \in \psetEfull,
    \end{align*}

    \item where step $(f)$ follows from 
    Lemma~\ref{sec:CheckCon:lem:integral w.r.t. psi dot e equals psi e},

    \item where step $(g)$ follows from the property of $ \mMLUf $ in~\eqref{sec:CheckCon:eqn:39} and the expression of $ \ZBSPA(\graphN) $ in~\eqref{sec:CheckCon:eqn:31},

    \item where step $(h)$ follows from the definition of $ \matr{C}_{\LCT{f}} $ in~\eqref{sec:LCT:eqn:6}.
\end{itemize}
