# Supplementary material for: Finite-Graph-Cover-Based Analysis of Factor Graphs in Classical and Quantum Information Processing Systems
Source: arXiv:2412.05942 source file (2024-12-08)
Supplement: Supplementary file 3 [file check_cond_upper.tex]

Consider the case where there exist $ e_{1} \in \setpf$ and $e_{2} \in \setpf $ such that
%------------------------------------------------------------------------
\begin{align}
    e_{1} \neq e_{2}, \qquad
    \LCTv{x}_{e_{1},e_{2}}' \defeq (\LCT{x}_{e_{1}}',\LCT{x}_{e_{2}}')
    \in \argmax_{ \LCTv{x}_{\psetpf \setminus \psetEf} }
    \bigl| 
        \vpsi_{ \psetpf \setminus \setEf }( \LCTv{x}_{\psetpf \setminus \setEf} ) 
    \bigr|.
    \label{sec:algsin:eqn:148}
      % \Biggl\{
      %   \Biggl(\prod_{e \in \setpf \setminus \setEf(\LCTv{x}_{\psetpf})} 
      %   |\cpsi_{e}(\LCT{x}_{e})| \Biggr) 
      %   \cdot \Biggl( \prod_{\upe \in \upsetpf \setminus \upsetEf(\LCTv{x}_{\psetpf}')}
      %   |\cpsi_{\upe}(\LCT{x}_{\upe}')| \Biggr)
      % \Biggr\}. 
\end{align}
%------------------------------------------------------------------------
The proof for other cases where there does not exists $ e_{1}, e_{2} \in \setpf $ satisfying~\eqref{sec:algsin:eqn:148} is similar and thus is omitted here. It holds that
%-----------------------------------------------------------------------
\begin{align}
  | \ZSSTLCTf(\cvpsi_{\psetpf}) | 
  % %--------------------------------------------------------------------
  &\overset{(a)}{=}  \left|\LCT{f}(\bm{0}) \cdot 
  \cvpsi_{\psetpf}(\bm{0})
  + \sum_{\LCTv{x}_{\psetpf}:\ \wh(\LCTv{x}_{\psetpf}) \geq 2} \LCT{f}(\LCTv{x}_{\psetpf}) 
  \cdot 
  \cvpsi_{\psetpf}(\LCTv{x}_{\psetpf})
  \right|
  \nonumber\\
  %--------------------------------------------------------------------
  &\leq \LCT{f}(\bm{0}) \cdot 
  |\cvpsi_{\psetpf}(\bm{0})|
  + \sum_{\LCTv{x}_{\psetpf}:\ \wh(\LCTv{x}_{\psetpf}) \geq 2} |\LCT{f}(\LCTv{x}_{\psetpf})| 
  \cdot |\cvpsi_{\psetpf}(\LCTv{x}_{\psetpf})|
  \nonumber \\
  %--------------------------------------------------------------------
  &\overset{(b)}{\leq} \LCT{f}(\bm{0}) \cdot 
  |\cvpsi_{\psetpf}(\bm{0})|
  + |\cvpsi_{\{e_{1},e_{2}\}}(\LCTv{x}_{e_{1},e_{2}}')|
  \cdot \sum_{\LCTv{x}_{\psetpf}:\ \wh(\LCTv{x}_{\psetpf}) \geq 2}
  |\LCT{f}(\LCTv{x}_{\psetpf})| \cdot |\cvpsi_{ \psetEf }( \LCTv{x}_{\psetEf} )|
  \nonumber\\
  %--------------------------------------------------------------------
  &\overset{(c)}{\leq} \LCT{f}(\bm{0}) \cdot 
  |\cvpsi_{\psetpf}(\bm{0})|
  + |\cvpsi_{\{e_{1},e_{2}\}}(\LCTv{x}_{e_{1},e_{2}}')|
  \cdot \sum_{\LCTv{x}_{\psetpf}:\ \wh(\LCTv{x}_{\psetpf}) \geq 2}
  |\LCT{f}(\LCTv{x}_{\psetpf})| \cdot |\cvpsi_{ \psetEf }( \LCTv{x}_{\psetEf} ) |^{1/(\df -2)}
  \nonumber\\
  %--------------------------------------------------------------------
  &\overset{(d)}{\leq} \LCT{f}(\bm{0}) \cdot 
  |\cvpsi_{\psetpf}(\bm{0})|
  + |\cvpsi_{\{e_{1},e_{2}\}}(\LCTv{x}_{e_{1},e_{2}}')|
  \cdot \sigupper( |\LCT{f}| )
  \nonumber\\
  %--------------------------------------------------------------------
  &\overset{(e)}{\leq} \LCT{f}(\bm{0}) \cdot 
  \bigl(
    |\cvpsi_{ \{e_{1},e_{2}\}}(\bm{0})| 
    + |\cvpsi_{ \{e_{1},e_{2}\} }(\LCTv{x}_{e_{1},e_{2}}')|
  \bigr) \nonumber\\
  %--------------------------------------------------------------------
  &\overset{(f)}{\leq} \LCT{f}(\bm{0}),
\end{align}
%-----------------------------------------------------------------------
where step $(a)$ follows from the expression of $ \ZSSTLCTf $ in~\eqref{sec:algsin:eqn:158} and the property that if $ \wh(\LCTv{x}_{\psetpf}) =1 $, we have $ \LCT{f}(\LCTv{x}_{\psetpf}) = 0 $ as stated in Proposition~\ref{prop:DENFG:LCT:1},
where step $(b)$ follows from~\eqref{sec:algsin:eqn:148}, \ie,
%----------------------------------------------------------------------------
\begin{align*}
  \sum_{\LCTv{x}_{\psetpf}:\ \wh(\LCTv{x}_{\psetpf}) \geq 2} |\LCT{f}(\LCTv{x}_{\psetpf})| 
  \cdot |\vpsi_{\psetpf}(\LCTv{x}_{\psetpf})|
  &\leq 
  \left\{
    \max_{ \LCTv{x}_{\psetpf \setminus \psetEf} }
    \bigl| 
        \vpsi_{ \psetpf \setminus \setEf }( \LCTv{x}_{\psetpf \setminus \setEf} ) 
    \bigr|
  \right\}
  \cdot
  \sum_{\LCTv{x}_{\psetpf}:\ \wh(\LCTv{x}_{\psetpf}) \geq 2} |\LCT{f}(\LCTv{x}_{\psetpf})| 
  \cdot |\vpsi_{\psetEf}(\LCTv{x}_{\psetEf})|
  \nonumber\\
  &= 
  |\cvpsi_{\{e_{1},e_{2}\}}(\LCTv{x}_{e_{1},e_{2}}')|
  \cdot
  \sum_{\LCTv{x}_{\psetpf}:\ \wh(\LCTv{x}_{\psetpf}) \geq 2} |\LCT{f}(\LCTv{x}_{\psetpf})| 
  \cdot |\vpsi_{\psetEf}(\LCTv{x}_{\psetEf})|,
\end{align*}
%----------------------------------------------------------------------------
where step $(c)$ follows from the fact that $ \df \geq 4 $ 
and 
$  0 \leq |\cpsi_{e}(\LCT{x}_{e})|, |\cpsi_{\upe}(\LCT{x}_{\upe})| \leq 1 $ for all $ \LCTv{x}_{\pe} \in \LCTset{X}_{\pe} $ and $ \pe \in \psetpf $,
where step $(d)$ follows from the definition of $ \sigupper $ in Definition~\ref{sec:algsin:def:1},
where step $(e)$ follows from the assumption in~\eqref{sec:3:eqn:13}, 
and where step $(f)$ follows from the Cauchy-Schwarz inequality, \ie,
%----------------------------------------------------------------------------
\begin{align*}
  |\cvpsi_{\{e_{1},e_{2}\}}(\bm{0})| 
  + |\cvpsi_{\{e_{1},e_{2}\}}(\LCTv{x}_{e_{1},e_{2}}')|
  \leq
  \Bigl( 
  \bigl| \cpsi_{e_{1}}(0) \bigr|^{2}
  +
  \bigl| \cpsi_{e_{1}}(\LCT{x}_{e_{1}}') \bigr|^{2} 
  \Bigr)^{1/2}
  \cdot 
  \Bigl( 
  \bigl| \cpsi_{e_{2}}(0) \bigr|^{2}
  +
  \bigl| \cpsi_{e_{2}}(\LCT{x}_{e_{2}}') \bigr|^{2} 
  \Bigr)^{1/2}
  \leq 1, \qquad 
  \| \cvpsi_{e_{1}} \|_{2} = \| \cvpsi_{e_{2}} \|_{2} =1.
\end{align*}
