# Supplementary material for: Finite-Graph-Cover-Based Analysis of Factor Graphs in Classical and Quantum Information Processing Systems
Source: arXiv:2412.05942 source file (2024-12-08)
Supplement: Supplementary file 4 [file checkable_cond_graphcover.tex]

In this appendix, we prove Theorem~\ref{sec:CheckCon:thm:1}.
By the analysis above Theorem~\ref{sec:CheckCon:thm:1}, it is sufficient to prove that~\eqref{sec:CheckCon:eqn:17}, \text{i.e.}, 
%----------------------------------------------------------------------------
\begin{align*}
    \lim_{M \to \infty} \Biggl(
        \int 
        \ZSSTM(\LCTavgalt{\graphN},\cvpsiavgalt)
        \dd{\muFSsimple(\cvpsiavgalt)}
    \Biggr)^{1/M}
    = \ZBSPA(\graphN)
\end{align*}
%----------------------------------------------------------------------------
holds under the condition
%---------------------------------------------------------------------------
\begin{align}
    \LCT{u}_{f}(\LCTvxf,0)
    = [\LCTvxf = \bm{0}], \quad 
    \LCTvxf \in \LCTset{X}_{\setpf}, \, f \in \setEfull,
    \label{sec:CheckCon:eqn:22}
\end{align}
%---------------------------------------------------------------------------
where the set $ \LCTset{X}_{\setpf} = \prod_{e} \LCTset{X}_{e} $ and the variables 
%---------------------------------------------------------------------------
\begin{align}
    \LCTv{x}_{\psetpf} &= (\LCT{x}_{\pe})_{\pe \in \psetpf} 
    = ( \LCTv{x}_{\setpf}, \LCTv{x}_{\upsetpf} )
    \in \LCTset{X}_{\psetpf},\quad
    \LCTv{x}_{\setpf} = (\LCT{x}_{e})_{e \in \setpf}, 
    \in \LCTset{X}_{\setpf}, \qquad
    \LCTv{x}_{\upsetpf} 
    = (\LCT{x}_{\upe})_{\upe \in \upsetpf}, 
    \in \LCTset{X}_{\upsetpf}, \nonumber\\
    \LCT{x}_{\pe} &= (\LCT{x}_{e}, \LCT{x}_{\upe}) 
    \in \LCTset{X}_{\pe}, \quad
    \LCT{x}_{e} \in \LCTset{X}_{e},\, \LCT{x}_{\upe} 
    \in \LCTset{X}_{\upe}, 
    \nonumber\\
    \LCTv{x}_{\psetpff} &= (\LCT{x}_{\pe,f})_{\pe \in \psetpf} 
    =  ( \LCTv{x}_{\setpf,f}, \LCTv{x}_{\upsetpf,f} )
    \in \LCTset{X}_{\psetpf}, 
    \quad
    \LCTv{x}_{\setpf,f} = (\LCT{x}_{e,f})_{e \in \setpf}, 
    \in \LCTset{X}_{\setpf}, \qquad
    \LCTv{x}_{\upsetpf,f} 
    = (\LCT{x}_{\upe,f})_{\upe \in \upsetpf}, 
    \in \LCTset{X}_{\upsetpf}, 
    \label{sec:CheckCon:eqn:27}\\
    \LCT{x}_{\pe,f} &= (\LCT{x}_{e,f}, \LCT{x}_{\upe,f}) 
    \in \LCTset{X}_{\pe}, \quad
    \LCT{x}_{e,f} \in \LCTset{X}_{e},\, \LCT{x}_{\upe,f} 
    \in \LCTset{X}_{\upe}. \label{sec:CheckCon:eqn:28}
\end{align}
%---------------------------------------------------------------------------
are defined in Definition~\ref{def:DENFG:LCT:1},
where $ \ZSSTM(\LCTavgalt{\graphN},\cvpsiavgalt) $ is defined in~\eqref{sec:CheckCon:eqn:8},
and where the functions $ \LCT{u}_{f} $ and $ \LCT{\lambda}_{f} $ are defined in~\eqref{sec:LCT:eqn:2}--\eqref{sec:LCT:eqn:3}.
Note that for each $ f \in \setF $, the largest eigenvalue for the matrix $ \LCTv{C}_{f} $ is $ \LCT{\lambda}_{f}(0) $ and the associated eigenvector is $ \LCTv{u}_{f}(0) $ as shown in~\eqref{sec:LCT:eqn:3}--\eqref{sec:LCT:eqn:7}. In the remaining part of this proof, we assume that $ \LCT{u}_{f} $ satisfies~\eqref{sec:CheckCon:eqn:22}. We have
%-----------------------------------------------------------------------
\begin{align}
    \ZBSPA(\graphN)
    &\overset{(a)}{=} 
    \ZBSPA(\LCT{\graphN},\LCT{\vmu})
    \nonumber\\
    &\overset{(b)}{=} 
    \frac{
        \prod_{f} \Bigl( 
        \sum_{\LCTv{x}_{\psetpf}} 
        \LCT{f}(\LCTv{x}_{\psetpf})
        \prod_{\pe \in \setpf}
        \LCT{\mu}_{\ef}^{(t)}(x_e)
        \cdot 
        \LCT{\mu}_{\upef}^{(t)}(x_{\upe})
        \Bigr)
    }{ 
        \prod_{e} 
        \Bigl( 
            \sum_{\xpe=(x_{e},x_{\upe})} 
            \LCT{\mu}_{\efi}^{(t)}(x_e)
            \cdot
            \LCT{\mu}_{\efj}^{(t)}(x_e)
            \cdot
            \LCT{\mu}_{\upefi}^{(t)}(x_{\upe})
            \cdot
            \LCT{\mu}_{\upefj}^{(t)}(x_{\upe}) 
        \Bigr) 
    } \nonumber\\
    &\overset{(c)}{=} \LCT{g}(\vect{0}) 
    \nonumber\\
    &\overset{(d)}{=}  
    \prod_{f \in \setF} \LCT{f}(\bm{0})
    \nonumber\\
    &\overset{(e)}{=} 
    \prod_{f \in \setF}
    \Biggl( 
        \sum_{\LCTellf \in \LCTset{L}_{f}}
            \LCT{\lambda}_{f}(\LCTellf) \cdot
            \LCT{u}_{f}(\bm{0},\LCTellf) 
        \cdot 
        \overline{ 
            \LCT{u}_{f}
            (\bm{0}, \LCTellf)
        }
    \Biggr) \nonumber\\
    &\overset{(f)}{=} \prod_{f \in \setF} \LCT{\lambda}_{f}(0),
    \label{sec:CheckCon:eqn:18}
\end{align}
%-----------------------------------------------------------------------
where step $(a)$ follows from the property of the SPA fixed-point messages vector in~\eqref{sec:CheckCon:eqn:31},
where step $(b)$ follows from the definition of $ \ZBSPA(\LCT{\graphN},\LCT{\vmu}) $ in Definition~\ref{sec:DENFG:def:3} and the fact that, as defined in item~\ref{def:DENFG:LCT:1:item:2} in Definition~\ref{def:DENFG:LCT:1}, in $ \LCT{\graphN} $ the local function associated with function node $ f $ is $ \LCT{f} $,
where step $(c)$ follows from the expressions of the fixed point messages $ \LCT{\vmu} $ in~\eqref{sec:CheckCon:eqn:7} and Property~\ref{prop:DENFG:LCT:1:item:4}\footnote{{\color{blue}XXXX If we replace the word Property with the word Item, then we need to change it gloally. XXXX}} in Proposition~\ref{prop:DENFG:LCT:1},
where step $ (d) $ follows from the global function $ \LCT{g}(\vx) = \prod_{f} \LCT{f}(\LCTv{x}_{f}) $ of $ \LCT{\graphN} $ as defined in Definition~\ref{def:DENFG:LCT:1},
where step $ (e) $ follows from the decomposition of $ \LCT{f} $ in Property~\ref{prop:DENFG:LCT:1:item:5} in Proposition~\ref{prop:DENFG:LCT:1}, where step $ (f) $ follows from
%-----------------------------------------------------------------------
\begin{align*}
    0
    &\overset{(f)}{=} \sum_{ 
      \LCTvxf 
      \in \LCTsetxpf
    }
    \LCT{u}_{f}(\LCTvxf,0) 
    \cdot 
    \overline{\LCT{u}_{f}
    (\LCTvxf,\ell_{\LCT{f}}')}
    \nonumber\\
    &\overset{(g)}{=}
    \overline{\LCT{u}_{f}
    (\bm{0},\ell_{\LCT{f}}')},
    \qquad 
    \ell_{\LCT{f}}' \in \LCTset{L}_{f} \setminus \{0\}, \,
    f \in \setF,
    \nonumber\\
    1&\overset{(f)}{=} \sum_{ 
      \LCTvxf 
      \in \LCTsetxpf
    }
    \LCT{u}_{f}(\LCTvxf,0) 
    \cdot 
    \overline{\LCT{u}_{f}
    (\LCTvxf,0)}
    \nonumber\\
    &\overset{(g)}{=}
    \overline{\LCT{u}_{f}
    (\bm{0},0)},\, f \in \setF,
\end{align*}
%-----------------------------------------------------------------------
where step $(f)$ follows from the definition of $ \LCT{u}_{f} $ and $ \LCTset{L}_{f} $ in~\eqref{sec:LCT:eqn:5} in Property~9 in Proposition~\ref{prop:DENFG:LCT:1},
and where step $(g)$ follows from the expression of $ \LCT{u}_{f}(\LCTvxf,0) $ in~\eqref{sec:CheckCon:eqn:22}. Steps $ (f) $ and $ (g) $ in the above expressions imply 
%---------------------------------------------------------------------------
\begin{align*}
    \begin{pmatrix}
        \LCT{u}_{f}(\bm{0},0) & \LCT{u}_{f}(\bm{0},1) & \cdots &
        \LCT{u}_{f}(\bm{0},|\LCTset{L}_{f}|)
    \end{pmatrix} = 
     \begin{pmatrix}
        1 & 0 & \cdots & 0
    \end{pmatrix}, \qquad f \in \setF.
\end{align*}
%---------------------------------------------------------------------------

The remaining part of the proof is divided into three parts.
%---------------------------------------------------------------------------
\begin{enumerate}
    \item We rewrite $ \ZSSTM(\LCTavgalt{\graphN},\cvpsiavgalt) $ in~\eqref{sec:CheckCon:eqn:8} as
    %-------------------------------------------------------------------
    \begin{align}
        \ZSSTM(\LCTavgalt{\graphN},\cvpsiavgalt)
        &\overset{(a)}{=}
        \prod_f \left( 
          \sum_{\LCTv{x}_{\psetpff}}
          \sum_{\LCTellf \in \LCTset{L}_{f}}
                \LCT{\lambda}_{f}(\LCTellf) \cdot
                \LCT{u}_{f}(\LCTv{x}_{\setpff},\LCTellf) 
            \cdot 
            \overline{ 
                \LCT{u}_{f}
                (\LCTv{x}_{\upsetpff}, \LCTellf)
            }
          \prod_{\pe \in \psetpf} 
          \cpsi_{\pe,f}(\LCT{x}_{\pe,f}) 
        \right)^{M}
        \nonumber\\
        &\overset{(b)}{=}
        \prod_f \left(
          \sum_{\LCTellf \in \LCTset{L}_{f}}
            \LCT{\lambda}_{f}(\LCTellf) 
            \cdot
            \Biggl( 
                \sum_{\LCTv{x}_{\setpff}}
                \LCT{u}_{f}(\LCTv{x}_{\setpff},\LCTellf) 
                \prod_{e \in \setpf} 
                \cpsi_{e,f}(\LCT{x}_{e,f}) 
            \Biggr)
            \cdot 
            \Biggl( 
                \sum_{\LCTv{x}_{\upsetpff}}
                \overline{ 
                    \LCT{u}_{f}
                    (\LCTv{x}_{\upsetpff}, \LCTellf)
                }
                \prod_{\upe \in \upsetpf} 
                \cpsi_{\upe,f}(\LCT{x}_{\upe,f}) 
             \Biggr)
        \right)^{M}, \label{sec:CheckCon:eqn:10}
    \end{align}
    %-------------------------------------------------------------------
    where step $(a)$ follows from the decomposition of $ \LCT{f} $ in~\eqref{sec:LCT:eqn:2},
    and where step $(b)$ follows from the definition of $ \cpsi_{\pe} $ in~\eqref{sec:SST:eqn:20}, \textit{i.e.}, $ \cpsi_{\pe,f}(\LCT{x}_{\pe,f})=  \cpsi_{e,f}(\LCT{x}_{e,f}) \cdot \cpsi_{\upe,f}(\LCT{x}_{\upe,f}) $ for all $ \LCT{x}_{\pe,f} = (\LCT{x}_{e,f},\LCT{x}_{\upe,f}) \in \LCTset{X}_{\pe} $ which is given in~\eqref{sec:CheckCon:eqn:28} with $ \LCTset{X}_{\pe} =  \LCTset{X}_{e}^{2} $ as defined in item~\ref{def:DENFG:LCT:1:item:5} in Definition~\ref{def:DENFG:LCT:1}, where the variable $ \LCTv{x}_{\psetpff} $ equals $ ( \LCTv{x}_{\setpff}, \LCTv{x}_{\upsetpff} ) $ as specified in~\eqref{sec:CheckCon:eqn:27}, and where the set $ \psetpf = \setpf \times \upsetpf $ is defined in item~\ref{sec:DENFG:def:4:item:2} in Definition~\ref{sec:DENFG:def:4}. Then $ |\ZSSTM(\LCTavgalt{\graphN},\cvpsiavgalt)| $ satisfies
    %-------------------------------------------------------------------
    \begin{align}
        &|\ZSSTM(\LCTavgalt{\graphN},\cvpsiavgalt)|
        \nonumber\\
        &\overset{(a)}{\leq}
        \prod_f \left( 
          \sum_{\LCTellf \in \LCTset{L}_{f}}
            \LCT{\lambda}_{f}(\LCTellf) 
            \cdot
            \Biggl| 
                \sum_{\LCTv{x}_{\setpff}}
                \LCT{u}_{f}(\LCTv{x}_{\setpff},\LCTellf) 
                \prod_{e \in \setpf} 
                \cpsi_{e,f}(\LCT{x}_{e,f}) 
            \Biggr|
            \cdot 
            \Biggl| 
                \sum_{\LCTv{x}_{\upsetpff}}
                \overline{ 
                    \LCT{u}_{f}
                    (\LCTv{x}_{\upsetpff}, \LCTellf)
                }
                \prod_{\upe \in \upsetpf} 
                \cpsi_{\upe,f}(\LCT{x}_{\upe,f}) 
             \Biggr|
        \right)^{M} \nonumber\\
        &\overset{(b)}{\leq}
        \prod_f \left( 
            \max_{
               \overset{\vpsi_{f},\vpsi_{f}' 
               \in \sC^{| \LCTsetxf|}}
               { \| \vpsi_{f} \|= \| \vpsi_{f}' \| = 1 }
            }
            \sum_{\LCTellf \in \LCTset{L}_{f}}
            \LCT{\lambda}_{f}(\LCTellf) 
            \cdot
            \Biggl| 
                \sum_{\LCTv{x}_{\setpff}}
                \LCT{u}_{f}(\LCTv{x}_{\setpff},\LCTellf) 
                \cdot \psi_{f}(\LCTv{x}_{\setpff})
            \Biggr|
            \cdot 
            \Biggl| 
                \sum_{\LCTv{x}_{\upsetpff}}
                \overline{ 
                    \LCT{u}_{f}
                    (\LCTv{x}_{\upsetpff}, \LCTellf)
                    \cdot \psi_{f}'(\LCTv{x}_{\upsetpff})
                }
             \Biggr|
        \right)^{M} 
        \nonumber\\
        &\overset{(c)}{\leq}
        \prod_f \left( 
            \max_{\LCTellf \in \LCTset{L}_{f}}
            \LCT{\lambda}_{f}(\LCTellf) 
        \right)^{M}
        \nonumber\\
        &\overset{(g)}{=}
        \prod_f \left( 
            \LCT{\lambda}_{f}(0) 
        \right)^{M} \label{sec:CheckCon:eqn:14}
    \end{align}
    %-------------------------------------------------------------------
    where step $(a)$ follows from $ \LCT{\lambda}_{f}(\LCTellf) \in \sR_{\geq 0} $ for all $ \LCTellf \in \LCTset{L}_{f} $ and $ f \in \setF $ as stated in Property 9 in Proposition~\ref{prop:DENFG:LCT:1},
    where step $ (b) $ follows from 
    %-------------------------------------------------------------------
    \begin{align*}
        \vpsi_{f} = \bigl(\psi_{f}(\LCTv{x}_{\setpff}) \bigr)_{\LCTv{x}_{\setpff} \in \LCTsetxpf} \in \sC^{|\LCTsetxpf|},
        \qquad
        \vpsi_{f}' = \bigl(\psi_{f}'(\LCTv{x}_{\setpff}) \bigr)_{\LCTv{x}_{\setpff} \in \LCTsetxpf} \in \sC^{|\LCTsetxpf|},
        \qquad 
        \|\vpsi_{f}\| = \| \vpsi_{f}' \|=1,
    \end{align*}
    %-------------------------------------------------------------------
    the definition of $ \LCTsetxpf $ in item~\ref{def:DENFG:LCT:1:item:1} in Definition~\ref{def:DENFG:LCT:1}, the definition of $ \cvpsi_{e} $ Definition~\ref{sec:SST:def:3} and the definition of $ \cvpsi_{e,f} $ in~\eqref{sec:SST:eqn:18}, \textit{i.e.}, $ \| \cpsi_{e,f} \| = 1 $ and $ \| \cpsi_{\upe,f} \| = 1 $ for all $ e \in \setpf $ and $ \upe \in \upsetpf $, 
    where step $(c)$ follows from 
    %----------------------------------------------------------------------------
    \begin{align}
        &\max_{
           \vpsi_{f},\vpsi_{f}' 
           \in \sC^{| \LCTsetxf|}
        }
        \sum_{\LCTellf \in \LCTset{L}_{f}}
        \LCT{\lambda}_{f}(\LCTellf) 
        \cdot
        \Biggl| 
            \sum_{\LCTv{x}_{\setpff}}
            \LCT{u}_{f}(\LCTv{x}_{\setpff},\LCTellf) 
            \cdot \psi_{f}(\LCTv{x}_{\setpff})
        \Biggr|
        \cdot 
        \Biggl| 
            \sum_{\LCTv{x}_{\upsetpff}}
            \overline{ 
                \LCT{u}_{f}
                (\LCTv{x}_{\upsetpff}, \LCTellf)
                \cdot \psi_{f}'(\LCTv{x}_{\upsetpff})
            }
        \Biggr|
        \label{sec:CheckCon:eqn:29}\\
        &\qquad \mathrm{s.t.}\quad 
        \|\vpsi_{f}\|= \|\vpsi_{f}'\|=1, 
        \nonumber\\
        &\overset{(d)}{=} \max_{
            \vpsi_{f} \in \sC^{|\LCTsetxf|}
        } \sum_{\LCTellf \in \LCTset{L}_{f}}
        \LCT{\lambda}_{f}(\LCTellf) 
        \cdot
        \Biggl| 
            \sum_{\LCTv{x}_{\setpff}}
            \LCT{u}_{f}(\LCTv{x}_{\setpff},\LCTellf) 
            \cdot \psi_{f}(\LCTv{x}_{\setpff})
        \Biggr|^{2}
        \nonumber\\
        &\qquad \mathrm{s.t.}\quad 
        \|\vpsi_{f}\|=1
        \nonumber\\
        &\overset{(e)}{=} \max_{
            \vpsi_{f} \in \sC^{| \LCTsetxf|}
        } \sum_{\LCTv{x}_{\psetpff}} 
        \LCT{f}(\LCTv{x}_{\setpff}, \LCTv{x}_{\upsetpff})
        \cdot \psi_{f}(\LCTv{x}_{\setpff})
        \cdot \overline{ \psi_{f}(\LCTv{x}_{\upsetpff}) }
        \nonumber\\
        &\qquad \mathrm{s.t.}\quad 
        \|\vpsi_{f}\|=1 \nonumber\\
        &\overset{(f)}{=} \max_{\LCTellf}
        \LCT{\lambda}_{f}(\LCTellf) 
    \end{align}
    %----------------------------------------------------------------------------
    where step $(d)$ follows from the following facts:
    %---------------------------------------------------------------------------
    \begin{enumerate}
        \item the function $  \LCT{\lambda}_{f}(\ellf) $ is nonnegative real-valued for all $ \ellf \in \LCTset{L}_{f} $ as defined in~\eqref{sec:LCT:eqn:3}; 

        \item by Cauchy-Schwarz inequality, the objective function in the optimization problem~\eqref{sec:CheckCon:eqn:29} is maximized when $ \cvpsi_{f}' = \overline{ \cvpsi_{f} } $,
    \end{enumerate}
    %---------------------------------------------------------------------------
    where step $(e)$ follows from the decompostion of $ \LCT{f} $ in~\eqref{sec:LCT:eqn:2}--\eqref{sec:LCT:eqn:3},
    where step $(f)$ follows from Courant–Fischer–Weyl min-max principle of the PSD matrix $ \LCTv{C}_{f} $ defined in~\eqref{sec:LCT:eqn:7}:
    %------------------------------------------------------------------------
    \begin{align*}
        \sum_{\LCTv{x}_{\psetpff}} 
        \LCT{f}(\LCTv{x}_{\setpff}, \LCTv{x}_{\upsetpff})
        \cdot \psi_{f}(\LCTv{x}_{\setpff})
        \cdot \overline{ \psi_{f}(\LCTv{x}_{\upsetpff}) }
        &= \vpsi_{f}^{\tran} \cdot \LCTv{C}_{f} \cdot
        \overline{ \vpsi_{f} }, \nonumber\\
        \max_{\LCTellf}
        \LCT{\lambda}_{f}(\LCTellf) &=\max_{
            \vpsi_{f} \in \sC^{| \LCTsetxf|}
        } \vpsi_{f}^{\tran} \cdot \LCTv{C}_{f} \cdot
        \overline{ \vpsi_{f} }
        \nonumber\\
        &\qquad \mathrm{s.t.}\quad 
        \|\vpsi_{f}\|=1,
    \end{align*}
    %------------------------------------------------------------------------
    and where step $(g)$ follows from the fact that $ \LCT{\lambda}_{f}(0) $ is the largest eigenvalue for $ \LCTv{C}_{f} $ as defined in~\eqref{sec:LCT:eqn:3} for each $ f \in \setF $:
    %-----------------------------------------------------------------------
    \begin{align*}
        \LCT{\lambda}_{f}(0) = \max_{\LCTellf}
        \LCT{\lambda}_{f}(\LCTellf).
    \end{align*}
    %-----------------------------------------------------------------------
    
    \item Similar to the proof of Proposition~\ref{sec:SST:prop:3}, we define
    %-------------------------------------------------------------------
    \begin{align*}
        \LCT{\ell}^{(M)} \defeq ( \LCTellfm )_{f \in \setF, m \in [M]}
        \in \prod_{f} \LCTset{L}_{f}^{M}.
    \end{align*}
    %-------------------------------------------------------------------
    Then it holds that
    %-------------------------------------------------------------------
    \begin{align}
        &\int 
        \ZSSTM(\LCTavgalt{\graphN},\cvpsiavgalt)
        \dd{\muFSsimple(\cvpsiavgalt)}
        \nonumber\\
        &\overset{(a)}{=} 
        \int 
        \prod_f \left( 
          \sum_{\LCTellf \in \LCTset{L}_{f}}
            \LCT{\lambda}_{f}(\LCTellf) 
            \cdot
            \Biggl( 
                \sum_{\LCTv{x}_{\setpff}}
                \LCT{u}_{f}(\LCTv{x}_{\setpff},\LCTellf) 
                \prod_{e \in \setpf} 
                \cpsi_{e,f}(\LCT{x}_{e,f}) 
            \Biggr)
            \cdot 
            \Biggl( 
                \sum_{\LCTv{x}_{\upsetpff}}
                \overline{ 
                    \LCT{u}_{f}
                    (\LCTv{x}_{\upsetpff}, \LCTellf)
                }
                \prod_{\upe \in \upsetpf} 
                \cpsi_{\upe,f}(\LCT{x}_{\upe,f}) 
             \Biggr)
        \right)^{M}
        \dd{\muFSsimple(\cvpsiavgalt)}
        \nonumber\\
        &=
        \sum_{\LCT{\ell}^{(M)} \in \prod_{f} \LCTset{L}_{f}^{M} }
        \int 
        \prod_{m=1}^{M} 
        \prod_f
        \Biggl( 
            \sum_{\LCTv{x}_{\setpf,m}}
            \LCT{u}_{f}(\LCTv{x}_{\setpff,m},\LCTellfm) 
            \prod_{e \in \setpf} 
            \cpsi_{e,f}(\LCT{x}_{e,f,m}) 
        \Biggr)
        \cdot 
        \Biggl( 
            \sum_{\LCTv{x}_{\upsetpff,m}}
            \overline{ 
                \LCT{u}_{f}
                (\LCTv{x}_{\upsetpff,m}, \LCTellfm)
            }
            \prod_{\upe \in \upsetpf} 
            \cpsi_{\upe,f}(\LCT{x}_{\upe,f,m}) 
         \Biggr)
        \dd{\muFSsimple(\cvpsiavgalt)}
        \nonumber\\
        &\quad \cdot \Biggl(\prod_{m=1}^{M} 
        \prod_f \LCT{\lambda}_{f}(\LCTellfm) \Biggr) 
        \nonumber\\
        &\overset{(b)}{=} 
        \sum_{\LCT{\ell}^{(M)} \in \prod_{f} \LCTset{L}_{f}^{M} }
        \int 
        \prod_{m=1}^{M} 
        \prod_f
        \Biggl( 
            \sum_{\LCTv{x}_{\setpf,m}}
            \LCT{u}_{f}(\LCTv{x}_{\setpff,m},\LCTellfm) 
            \prod_{e \in \setpf} 
            \cpsi_{e,f}(\LCT{x}_{e,f,m}) 
        \Biggr)
        \prod_{e \in \setEfull}
        \dd{\muFSsimple(\cvpsi_{e})}
        \nonumber\\
        &\quad \cdot 
        \int 
        \prod_{m=1}^{M} 
        \prod_f
        \Biggl( 
            \sum_{\LCTv{x}_{\upsetpff,m}}
            \overline{ 
                \LCT{u}_{f}
                (\LCTv{x}_{\upsetpff,m}, \LCTellfm)
            }
            \prod_{\upe \in \upsetpf} 
            \cpsi_{\upe,f}(\LCT{x}_{\upe,f,m}) 
         \Biggr)
        \prod_{\upe \in \upsetEfull}
        \dd{\muFSsimple(\cvpsi_{\upe})}
        \cdot \Biggl(\prod_{m=1}^{M} 
        \prod_f \LCT{\lambda}_{f}(\LCTellfm) \Biggr) 
        \nonumber\\
        &\overset{(c)}{=}
        \sum_{\LCT{\ell}^{(M)} \in \prod_{f} \LCTset{L}_{f}^{M} }
        \Biggl(\prod_{m=1}^{M} 
        \prod_f \LCT{\lambda}_{f}(\LCTellfm) \Biggr) 
        \cdot
        \Biggl| \int 
        \prod_{m=1}^{M} 
        \prod_f
        \Biggl( 
            \sum_{\LCTv{x}_{\setpf,m}}
            \LCT{u}_{f}(\LCTv{x}_{\setpff,m},\LCTellfm) 
            \prod_{e \in \setpf} 
            \cpsi_{e,f}(\LCT{x}_{e,f,m}) 
        \Biggr)
        \prod_{e \in \setEfull}
        \dd{\muFSsimple(\cvpsi_{e})}
        \Biggr|^{2}, \label{sec:CheckCon:eqn:11}
    \end{align}
    %-------------------------------------------------------------------
    where step $(a)$ follows from the expression of $ \ZSSTM  $ in~\eqref{sec:CheckCon:eqn:10},
    where step $(b)$ follows from fact that the measure for  $ \{ \cvpsi_{e} \}_{e \in \setEfull}$ is independent of the measure for $ \{ \cvpsi_{\upe} \}_{\upe \in \upsetEfull} $, as defined in items~\ref{sec:SST:def:7:item:1} and~\ref{sec:SST:def:7:item:2} in Definition~\ref{sec:SST:def:7},
    and the properties of $ \muFSsimple(\cvpsiavgalt) $ in~\eqref{sec:SST:eqn:29}, 
    and where step $(c)$ follows from similar derivations of the expression in~\eqref{sec:SST:eqn:34} in the proof of Proposition~\ref{sec:SST:prop:3}:
    %------------------------------------------------------------------------
    \begin{align*}
        &\int 
        \prod_{m=1}^{M} 
        \prod_f
        \Biggl(
            \sum_{\LCTv{x}_{\upsetpff,m}}
            \overline{ 
                \LCT{u}_{f}
                (\LCTv{x}_{\upsetpff,m}, \LCTellfm)
            }
            \prod_{\upe \in \upsetpf} 
            \cpsi_{\upe,f}(\LCT{x}_{\upe,f,m})    
        \Biggr)
        \prod_{\upe \in \upsetEfull}
        \dd{\muFSsimple(\cvpsi_{\upe})}
        \nonumber\\
        &\overset{(d)}{=} 
        \Biggl(\int 
        \prod_{m=1}^{M} 
        \prod_f
        \Biggl( 
            \sum_{\LCTv{x}_{\setpf,m}}
            \overline{
                \LCT{u}_{f}(\LCTv{x}_{\setpff,m},\LCTellfm) 
            }
            \prod_{e \in \setpf} 
            \cpsi_{e,f}(\LCT{x}_{e,f,m})
        \Biggr)
        \prod_{e \in \setEfull}
        \dd{\muFSsimple(\cvpsi_{e})}
        \nonumber\\
        &= \overline{ 
        \Biggl(\int 
            \prod_{m=1}^{M} 
            \prod_f
            \Biggl( 
                \sum_{\LCTv{x}_{\setpf,m}}
                \LCT{u}_{f}(\LCTv{x}_{\setpff,m},\LCTellfm) 
                \prod_{e \in \setpf} 
                \overline{ \cpsi_{e,f}(\LCT{x}_{e,f,m}) }
            \Biggr)
            \prod_{e \in \setEfull}
            \dd{\muFSsimple(\cvpsi_{e})}
        }\Biggr)
        \nonumber\\
        &\overset{(e)}{=} \overline{ 
        \Biggl(\int 
        \prod_{m=1}^{M} 
        \prod_f
        \Biggl( 
            \sum_{\LCTv{x}_{\setpf,m}}
            \LCT{u}_{f}(\LCTv{x}_{\setpff,m},\LCTellfm) 
            \prod_{e \in \setpf} 
            \cpsi_{e,f}(\LCT{x}_{e,f,m})
        \Biggr)
        \prod_{e \in \setEfull}
        \dd{\muFSsimple(\cvpsi_{e})}
        \Biggr)}
    \end{align*}
    %------------------------------------------------------------------------
    where step $(d)$ follows from the following facts:
    %---------------------------------------------------------------------------
    \begin{enumerate}

        \item the properties of the SST in Section~\ref{sec:SST} still hold if we conisder applying the LCT and then the SST on a PE-NFG. In order to use the properties of the SST for the resulting PE-NFG, we need to do the following changes:
        %---------------------------------------------------------------------------
        \begin{itemize}
            \item for each $ \pe = (e,\upe) \in \psetEfull $, we replace $ \setxpe $, $ \setxe $, and $ \set{X}_{\upe} $ with $ \LCTset{X}_{\pe} $, $ \LCTsetxe $, and $ \LCTset{X}_{\upe} $, respectively;

            \item for each $ \pe = (e,\upe) \in \psetEfull $, we replace $ \xpe $, $ \xe $, and $ \xupe $ with $ \LCTv{x}_{\pe} $, $ \LCT{x}_{e} $, and $ \LCT{x}_{\upe} $, respectively; 

            \item for each $ f \in \setF $, we replace $ f $, $ u_{f} $, and $ \lambda_{f} $ with $ \LCT{f} $, $ \LCT{u}_{f} $, and $ \LCT{\lambda}_{f} $ which are defined in~\eqref{sec:LCT:eqn:1} and~\eqref{sec:LCT:eqn:2}--\eqref{sec:LCT:eqn:3}, respectively;

            \item for each $ f \in \setF $, we replace $ \vx_{\psetpff} $, $ \vx_{\setpf,f} $, and $ \vx_{\upsetpf,f} $ with $ \LCTv{x}_{\psetpff} $, $ \LCTv{x}_{\setpf,f} $, and $ \LCTv{x}_{\upsetpf,f} $, respectively;

            \item in terms of other variables, e.g., $ \vx_{\pe,m} $, $ x_{e,m} $, $  $, and $ x_{\upe,m} $ for each $ \pe = (e,\upe) \in \psetEfull $ and $ \vx_{\psetpff,m} $, $ \vx_{\setpf,f,m} $, and $ \vx_{\upsetpf,f,m} $ for $ f \in \setF $ with $ m \in \sZpp $, we the apply similar change as above,

        \end{itemize}
        %---------------------------------------------------------------------------

        \item for each $ f \in \setF $, the variables $ \LCTv{x}_{\setpff,m} $ and $ \LCTv{x}_{\upsetpff,m} $ defined in~\eqref{sec:CheckCon:eqn:27} have the same alphabet $\LCTsetxf = \prod_{e \in \setpf} \LCTsetxe =  \prod_{\upe \in \upsetpf} \LCTset{X}_{\upe} = \LCTset{X}_{\upsetpf} $ with $ \LCTsetxe = \LCTset{X}_{\upe} $ for all $ \pe = (e,\upe) \in \psetEfull $ as stated in item~\ref{def:DENFG:LCT:1:item:1} in Definition~\ref{def:DENFG:LCT:1};  

        \item for each $ \pe = (e,\upe) \in \psetEfull $, both $ \cvpsi_{e} $ and $ \cvpsi_{\upe} $ are vectors in $ \sC^{|\LCTsetxe|} $ with $ \|\cvpsi_{e}\| = \|\cvpsi_{\upe}\| =1 $;

        \item for each $ \pe= (e,\upe) \in \psetEfull $, both the measure $ \dd{\muFSsimple(\cvpsi_{e})} $ and the measure $ \dd{\muFSsimple(\cvpsi_{\upe})} $ are independent Fubini-Study measures, \textit{i.e.}, Haar measures over $ \sC^{|\LCTsetxe|} $, which are defined following the similar idea in~\eqref{sec:SST:eqn:30}, 

    \end{enumerate}
    %---------------------------------------------------------------------------
    and where step $(e)$ again follows from the fact that for each $ e \in \setEfull $, the measure $ \dd{\muFSsimple(\cvpsi_{e})} $ is a Fubini-Study measure, \textit{i.e.}, a Haar measure over $ \sC^{|\LCTsetxe|} $. 
    % and where step $(f)$ follows from Assumption~\ref{sec:DENFG:asum:2}, Property 8 in Proposition~\ref{prop:DENFG:LCT:1} and the fact that $ \LCT{\lambda}_{f}(\ellf) \in \sR_{\geq 0} $ for all $ \ellf \in \set{L}_{f} $ and $ f \in \setF $ as defined in~\eqref{sec:LCT:eqn:2}--\eqref{sec:LCT:eqn:3}. }
    Then we have
    %-------------------------------------------------------------------
    \begin{align}
        \int 
        \ZSSTM(\LCTavgalt{\graphN},\cvpsiavgalt)
        \dd{\muFSsimple(\cvpsiavgalt)} 
        &\overset{(a)}{\geq}
        \Bigl(\prod_{m=1}^{M} 
        \prod_f \LCT{\lambda}_{f}(0) \Bigr) 
        \cdot
        \Biggl| \int 
        \prod_{m=1}^{M} 
        \prod_f
        \Biggl( 
            \sum_{\LCTv{x}_{\setpf,m}}
            \LCT{u}_{f}(\LCTv{x}_{\setpff,m},0) 
            \prod_{e \in \setpf} 
            \cpsi_{e,f}(\LCT{x}_{e,f,m}) 
        \Biggr)
        \dd{\muFSsimple(\cvpsiavgalt)}
        \Biggr|^{2} \nonumber\\
        &\overset{(b)}{=} 
        \Bigl(
            \prod_f \LCT{\lambda}_{f}(0) 
        \Bigr)^{M}
        \cdot
        \Biggl| \int 
        \prod_{m=1}^{M} 
        \prod_f
        \prod_{e \in \setpf} 
        \cpsi_{e,f}(0) 
        \dd{\muFSsimple(\cvpsiavgalt)}
        \Biggr|^{2} \nonumber\\
        &\overset{(c)}{=} 
        \Bigl(
            \prod_f \LCT{\lambda}_{f}(0) 
        \Bigr)^{M}
        \prod_{e = (f_{i},f_{j}) \in \setEfull}
        \Biggl( 
            \int 
            \prod_{m=1}^{M} 
            \Bigl( 
                \cpsi_{e,f_{i}}(0) \cdot \cpsi_{e,f_{j}}(0) 
            \Bigr)
            \dd{\muFSsimple(\cvpsiavgalt)}
        \Biggr)^{2}
        \nonumber\\
        &\overset{(d)}{=}
        \Bigl(
            \prod_f \LCT{\lambda}_{f}(0) 
        \Bigr)^{M}
        \prod_{e = (f_{i},f_{j}) \in \setEfull}
        \Biggl( 
            \int 
            |\cpsi_{e,f_{i}}(0)|^{2M} 
            \dd{\muFSsimple(\cvpsiavgalt)}
        \Biggr)^{2}
        \nonumber\\
        &\overset{(e)}{=} \Bigl(
            \prod_f \LCT{\lambda}_{f}(0) 
        \Bigr)^{M}
        \cdot
        \prod_{e \in \setEfull}
        \frac{1}{|\set{B}_{\LCTset{X}_e^M}|^{2}} 
        \label{sec:CheckCon:eqn:15}
    \end{align}
    %-------------------------------------------------------------------
    where step $(a)$ follows from the expression of $ \int 
        \ZSSTM(\LCTavgalt{\graphN},\cvpsiavgalt)
        \dd{\muFSsimple(\cvpsiavgalt)}  $ in~\eqref{sec:CheckCon:eqn:11} and the fact that $ \LCT{\lambda}_{f}(\LCTellf) \in \sR_{\geq 0} $ for all $ \LCTellf \in \LCTset{L}_{f} $ and $ f \in \setF $ as defined in~\eqref{sec:LCT:eqn:3},
    where step $(b)$ follows from the expression of $ \LCT{u}_{f}(\LCTvxf,0) $ in~\eqref{sec:CheckCon:eqn:22}, 
    where step $(c)$ follows from the fact that the entries in $ \{ \cpsi_{\efi}(0)  \}_{e=(f_{i}, f_{j}) \in \setEfull} $ are independent and the entries in $ \{ \cpsi_{\efj}(0)  \}_{e=(f_{i}, f_{j}) \in \setEfull} $ are independent,  as defined in item~\ref{sec:SST:def:7:item:1} in Definition~\ref{sec:SST:def:7},
    where step $(d)$ follows from the definition of $  \cpsi_{e,f_{i}}(0) $ and $ \cpsi_{e,f_{j}}(0)  $ in~\eqref{sec:SST:eqn:18} and~\eqref{sec:SST:eqn:22}, \textit{i.e.}, $ \cpsi_{e,f_{i}}(0) = \cpsi_{e}(0) = \overline{ \cpsi_{e,f_{j}}(0)  }  $ for $ e = (f_{i},f_{j}) $, $ i < j $,
    and where step $(e)$ follows from~\eqref{sec:SST:eqn:25} in the proof of Proposition~\ref{sec:SST:prop:2}.
    
    \item Combining the results obtained above, we have
    %-------------------------------------------------------------------
    \begin{align*}
        \Bigl(
            \prod_f \LCT{\lambda}_{f}(0) 
        \Bigr)^{M}
        \cdot
        \prod_{e \in \setEfull}
        \frac{1}{|\set{B}_{\set{X}_e^M}|^{2}} 
        \overset{(a)}{\leq}
        \int 
        \ZSSTM(\LCTavgalt{\graphN},\cvpsiavgalt)
        \dd{\muFSsimple(\cvpsiavgalt)} 
        \overset{(b)}{\leq}
        \int 
        \prod_f \left( 
            \LCT{\lambda}_{f}(0) 
        \right)^{M}
        \dd{\muFSsimple(\cvpsiavgalt)}
        \overset{(c)}{=}
        \prod_f \left( 
            \LCT{\lambda}_{f}(0) 
        \right)^{M}.
    \end{align*}
    %-------------------------------------------------------------------
    where step $(a)$ follows from~\eqref{sec:CheckCon:eqn:15},
    where step $(b)$ follows from~\eqref{sec:CheckCon:eqn:14},
    where step $(c)$ follows from the fact that $ \dd{\muFSsimple(\cvpsiavgalt)} $ is a Fubini-Study measure, i.e, a Haar measure, satisfying
    %-----------------------------------------------------------------------
    \begin{align*}
        \int 
        \prod_f \left( 
            \LCT{\lambda}_{f}(0) 
        \right)^{M}
        \dd{\muFSsimple(\cvpsiavgalt)}
        =  \prod_f \Biggl( \left( 
            \LCT{\lambda}_{f}(0) 
        \right)^{M} \int 
        \dd{\muFSsimple(\cvpsiavgalt)}
        \Biggr) 
        \overset{(d)}{=} \prod_f \left( 
            \LCT{\lambda}_{f}(0) 
        \right)^{M}.
    \end{align*}
    %-----------------------------------------------------------------------
    where step $(d)$ follows from
    %-----------------------------------------------------------------------
    \begin{align*}
        \dd{\muFSsimple(\cvpsiavgalt)}
        &=\prod_{e \in \setEfull}
        \dd{\muFSsimple(\cvpsi_{e})}
        \cdot 
        \prod_{\upe \in \upsetEfull}
        \dd{\muFSsimple(\cvpsi_{\upe})}, \qquad 
        \int \dd{\muFSsimple(\cvpsi_{e})} = 
        \int \dd{\muFSsimple(\cvpsi_{\upe})} =1, \qquad 
        \pe = (e,\upe) \in \setEfull, \nonumber\\
        \int \dd{\muFSsimple(\cvpsiavgalt)}
        &= \Biggl( \prod_{e \in \setEfull} \int \dd{\muFSsimple(\cvpsi_{e})} \Biggr)
        \cdot \Biggl(\prod_{\upe \in \upsetEfull} \int \dd{\muFSsimple(\cvpsi_{\upe})} \Biggr)
        =1.
    \end{align*}
    %-----------------------------------------------------------------------
    Then we have
    %-------------------------------------------------------------------
    \begin{align*}
        \limsup_{M \to \infty}
        \left( \int 
        \ZSSTM(\LCTavgalt{\graphN},\cvpsiavgalt)
        \dd{\muFSsimple(\cvpsiavgalt)} 
        \right)^{1/M}
        \geq \limsup_{M \to \infty} 
        \Biggl(
            \Bigl(
                \prod_f \LCT{\lambda}_{f}(0) 
            \Bigr)
            \cdot
            \prod_{e \in \setEfull}
            \frac{1}{|\set{B}_{\LCTset{X}_e^M}|^{2/M}} 
        \Biggr)
        \overset{(a)}{=}  
        \prod_f \LCT{\lambda}_{f}(0),
    \end{align*}
    %-------------------------------------------------------------------
    where step $(a)$ follows from Lemma~\ref{sec:SST:lem:3}. Moreover, we have
    %-------------------------------------------------------------------
    \begin{align*}
        \limsup_{M \to \infty}
        \Biggl( \int 
        \ZSSTM(\LCTavgalt{\graphN},\cvpsiavgalt)
        \dd{\muFSsimple(\cvpsiavgalt)} 
        \Biggr)^{1/M}
        \leq 
        \prod_f 
        \LCT{\lambda}_{f}(0).
    \end{align*}
    %-------------------------------------------------------------------
    Combining the above two inequalities, we obtain
    %-------------------------------------------------------------------
    \begin{align*}
        \limsup_{M \to \infty}
        \Biggl( \int 
        \ZSSTM(\LCTavgalt{\graphN},\cvpsiavgalt)
        \dd{\muFSsimple(\cvpsiavgalt)} 
        \Biggr)^{1/M}
        = \prod_f 
        \LCT{\lambda}_{f}(0).
    \end{align*}
    %-------------------------------------------------------------------
\end{enumerate}
%---------------------------------------------------------------------------
Combining with the expression of $ \ZBSPA(\graphN) $ in~\eqref{sec:CheckCon:eqn:18}, we have
%-----------------------------------------------------------------------
\begin{align}
    \lim_{M \to \infty}
    \Biggl( \int 
    \ZSSTM(\LCTavgalt{\graphN},\cvpsiavgalt)
    \dd{\muFSsimple(\cvpsiavgalt)} 
    \Biggr)^{1/M}
    =  \ZBSPA(\graphN). \label{sec:CheckCon:eqn:20}
\end{align}
%-----------------------------------------------------------------------
Then we have
%-----------------------------------------------------------------------
\begin{align*}
    \lim_{M \to \infty}
    \ZBM(\LCT{\graphN}) 
    &\overset{(a)}{=}
    \lim_{M \to \infty}
    \left(
        \prod_{e \in \setEfull}
            |\set{B}_{\LCTset{X}_{e}^M}|
    \right)^{2/M}
    \cdot
    \Biggl(
        \int 
         \ZSSTM(\LCTavgalt{\graphN},\cvpsiavgalt)
        \dd{\muFSsimple(\cvpsiavgalt)}
    \Biggr)^{1/M} \nonumber\\
    &\overset{(b)}{=}
    \lim_{M \to \infty}
    \left(
        \prod_{e \in \setEfull}
            |\set{B}_{\LCTset{X}_{e}^M}|
    \right)^{2/M}
    \cdot 
    \lim_{M \to \infty}
    \Biggl(
        \int 
         \ZSSTM(\LCTavgalt{\graphN},\cvpsiavgalt)
        \dd{\muFSsimple(\cvpsiavgalt)}
    \Biggr)^{1/M} \nonumber\\
    &\overset{(c)}{=} \ZBSPA(\graphN),
\end{align*}
%-----------------------------------------------------------------------
where step $(a)$ follows from~\eqref{sec:CheckCon:eqn:19},
and where steps $(b)$ and $ (c) $ follow from Lemma~\ref{sec:SST:lem:3} and the expression in~\eqref{sec:CheckCon:eqn:20}.
