# Supplementary material for: Finite-Graph-Cover-Based Analysis of Factor Graphs in Classical and Quantum Information Processing Systems
Source: arXiv:2412.05942 source file (2024-12-08)
Supplement: Supplementary file 5 [file convergence_tensor_norm.tex]

Similar to the proof of Lemma~\ref{sec:algsin:lem:8}, we know that the sequence $ \left\{ \log( \Zabsf\left( \Bigl( \vgam_{\psetpf}^{(k)} \Bigr)^{1/\qf} \right) ) \right\}_{k \in \sZpp} $ converges. 
For fixed $ e' \in \setpf $, we consider a vector $ \vgam_{\psetpf,*}^{(k)} $ to be
%----------------------------------------------------------------------------
\begin{align*}
    \gamma_{e,*}^{(k)}(\xe) \defeq
    \begin{cases}
        \gamma_{e}^{(k)}(\xe) + \gamma_{e}^{*}(\xe) & e = e' \\
        \gamma_{e}^{(k)}(\xe) & \text{Otherwise}
    \end{cases}
\end{align*}
%----------------------------------------------------------------------------
Then we have
%----------------------------------------------------------------------------
\begin{align*}
    \left( 
        \left. 
            \nabla_{ \vgam_{\psetpf} } 
            \log( \Zabsfn\Bigl( (\vgam_{\psetpf} )^{1/\qf} \Bigr) )
        \right|_{ \vgam_{\psetpf} = \vgam_{\psetpf,*}^{(k)}  }
    \right)^{\tran}
    \cdot 
    \left( \vgam_{\psetpf}^{(k)} - \vgam_{\psetpf,*}^{(k)} \right)
    = -\sum_{\xep}
    \left. \pdv{}{ \gamma_{e'}(\xep) }
    \log( \Zabsfn( (\vgam_{\psetpf} )^{1/\qf} ) )
    \right|_{ \vgam_{\psetpf} = \vgam_{\psetpf}^{(k)}  } 
    \cdot \gamma_{e}^{*}(\xe)
    \cdot ( \frac{ \gamma_{e}^{(k)}(\xe) }{ 
     \gamma_{e}^{(k)}(\xe) +  \gamma_{e}^{*}(\xe) } 
\end{align*}
%----------------------------------------------------------------------------
By Proposition~\ref{sec:algsin:prop:5}, we know that the function $ \log( \Zabsfn\Bigl( (\vgam_{\psetpf} )^{1/\qf} \Bigr) ) $ is concave w.r.t. $ \vgam_{\psetpf} $. Thus the following inequality holds
%------------------------------------------------------------------------
\begin{align}
    &\log( \Zabsfn\Bigl( (\vgam_{\psetpf}^{*} )^{1/\qf} \Bigr) )
    \nonumber\\
    &\leq \log( \Zabsfn\Bigl( (\vgam_{\psetpf}^{(k)} )^{1/\qf} \Bigr) )
    + \left( 
        \left. 
            \nabla_{ \vgam_{\psetpf} } 
            \log( \Zabsfn\Bigl( (\vgam_{\psetpf} )^{1/\qf} \Bigr) )
        \right|_{ \vgam_{\psetpf} = \vgam_{\psetpf}^{(k)}  }
    \right)^{\tran}
    \cdot 
    \left( \vgam_{\psetpf}^{*} - \vgam_{\psetpf}^{(k)} \right) 
    \nonumber\\
    &= \log( \Zabsfn\Bigl( (\vgam_{\psetpf}^{(k)} )^{1/\qf} \Bigr) )
    +
    \sum_{e \in \setpf}
    \sum_{\xe}
    \left. \pdv{}{ \gamma_{e}(\xe) }
    \log( \Zabsfn( (\vgam_{\psetpf} )^{1/\qf} ) )
    \right|_{ \vgam_{\psetpf} = \vgam_{\psetpf}^{(k)}  } 
    \cdot \Bigl( 
        \gamma_{e}^{*}(\xe) - \gamma_{e}^{(k)}(\xe) 
    \Bigr)\nonumber\\
    & \quad
    +
    \sum_{\upe \in \upsetpf}
    \sum_{\xupe}
    \left. \pdv{}{ \gamma_{\upe}(\xupe) }
    \log( \Zabsfn( (\vgam_{\psetpf} )^{1/\qf} ) )
    \right|_{ \vgam_{\psetpf} = \vgam_{\psetpf}^{(k)}  } 
    \cdot \Bigl( 
        \gamma_{\upe}^{*}(\xupe) - \gamma_{\upe}^{(k)}(\xupe) 
    \Bigr)
    , 
    \qquad
    k \in \sZpp, \label{sec:algsin:eqn:104}
\end{align}
%------------------------------------------------------------------------
where the elements in the gradient $ \nabla_{ \vgam_{\psetpf} } 
    \log( \Zabsfn\Bigl( (\vgam_{\psetpf} )^{1/\qf} \Bigr) ) $ are given by
%------------------------------------------------------------------------
\begin{align}
    \left. \pdv{}{ \gamma_{e}(\xe) }
    \log( \Zabsfn( (\vgam_{\psetpf} )^{1/\qf} ) )
    \right|_{ \vgam_{\psetpf} = \vgam_{\psetpf}^{(k)}  }
    &= \frac{1}{\qe}
    \cdot \Biggl( 
    \frac{ 1
    }{ \bigl( \gamma_{e}^{(k)}(\xe) \bigr)^{(q-1)/q} }
    \cdot 
    \frac{ \gamet^{(k+1)}(\xe) }{ \sum_{\xe} 
        ( \gamma_{e}^{(k)}(\xe) )^{1/q} 
        \cdot \gamet^{(k+1)}(\xe) 
    }
    - 1 \Biggr), \label{sec:algsin:eqn:108}\\
    \left. \pdv{}{ \gamma_{\upe}(\xupe) }
    \log( \Zabsfn( (\vgam_{\psetpf} )^{1/\qf} ) )
    \right|_{ \vgam_{\psetpf} = \vgam_{\psetpf}^{(k)}  }
    &= \frac{1}{\qupe}
    \cdot \Biggl( 
    \frac{ 1
    }{ \bigl( \gamma_{\upe}^{(k)}(\xupe) \bigr)^{(q-1)/q} }
    \cdot 
    \frac{ \gamupet^{(k+1)}(\xupe) 
    }{ \sum_{\xe} 
        ( \gamma_{\upe}^{(k)}(\xupe) )^{1/q} 
        \cdot \gamupet^{(k+1)}(\xupe) 
    }
    - 1 \Biggr), \label{sec:algsin:eqn:124}
\end{align}
%------------------------------------------------------------------------
and $ \gamet^{(k+1)} $ and $ \gamupet^{(k+1)} $ are defined in~\eqref{sec:algsin:eqn:90} and~\eqref{sec:algsin:eqn:121}, respectively.  By Remark~\ref{sec:algsin:remk:1} and the fact that $ \gamma_{e}^{(0)}(\xe), \gamma_{\upe}^{(0)}(\xupe) \in \sR_{>0} $ for all $ \xpe \in \setxpe $ and $ \pe \in \psetpf $, we have $ \gamma_{e}^{(k)}(\xe), \gamet^{(k+1)}(\xe), \gamma_{\upe}^{(k)}(\xupe), \gamupet^{(k+1)}(\xupe) \in \sR_{>0} $ for all $ k \in \sZpp $, $ \xpe \in \setxpe $, and $ \pe \in \setpf $. Thus the partial derivatives in~\eqref{sec:algsin:eqn:108} and~\eqref{sec:algsin:eqn:124} are well defined.
Then we have
%------------------------------------------------------------------------
\begin{align}
    &\lim_{k \to \infty} \left. \pdv{}{ \gamma_{e}(\xe) }
    \log( \Zabsfn( (\vgam_{\psetpf} )^{1/\qf} ) )
    \right|_{ \vgam_{\psetpf} = \vgam_{\psetpf}^{(k)}  } 
    \cdot \gamma_{e}^{(k)}(\xe) 
    \nonumber\\
    &=\lim_{k \to \infty}
    \left( \gamma_{e}^{(k)}(\xe) \right)^{1/\qe} 
    \cdot
    \Biggl( 
    \frac{ \gamet^{(k+1)}(\xe) }{ \sum_{\xe} 
        \left( \gamma_{e}^{(k)}(\xe) \right)^{1/\qe} 
        \cdot \gamet^{(k+1)}(\xe) 
    }
    - \bigl( \gamma_{e}^{(k)}(\xe) \bigr)^{(\qe-1)/\qe} \Biggr)
    \nonumber\\
    &\overset{(a)}=  0, \qquad \xe \in \setxe, \, e \in \setpf,
    \label{sec:algsin:eqn:110}
\end{align}
%------------------------------------------------------------------------
where step $(a)$ follows from Lemma~\ref{sec:algsin:lem:4} with the substitution in~\eqref{sec:algsin:eqn:4} and the fact that $ \| \vgam_{e}^{(k)} \|_{q} = 1 $, i.e., $ \{ \gamma_{e}^{(k)}(\xe) \}_{k \in \sZpp} $ is a bounded sequence. Because the sequences $ \{\gamma_{e}^{(k)}(\xe)\}_{k \in \sZpp} $ and  $ \{\gamma_{\upe}^{(k)}(\xupe)\}_{k \in \sZpp} $ are bounded for all $ \xpe \in \setx_{\pe} $ and $ \pe = (e,\upe) \in \psetEfull $, we define the sets
%------------------------------------------------------------------------
\begin{align*}
    \set{S}_{e,1} & \defeq \left\{ \xe \in \setxe  
    \ \left| \ \liminf_{k \to \infty} \gamma_{e}^{(k)}(\xe) > 0 
    \right. \right\}, \qquad
    \set{S}_{e,1}^{\mathrm{c}} \defeq \setxe \setminus \set{S}_{e,1},
    \nonumber\\
    \set{S}_{\upe,1} & \defeq \left\{ \xupe \in \setx_{\upe}  
    \ \left| \ \liminf_{k \to \infty} \gamma_{\upe}^{(k)}(\xupe) > 0 
    \right. \right\}, \qquad 
    \set{S}_{\upe,1}^{\mathrm{c}} \defeq \setxe \setminus \set{S}_{\upe,1},
\end{align*}
%------------------------------------------------------------------------
which implies
%----------------------------------------------------------------------------
\begin{align}
    \liminf_{k \to \infty} \gamma_{e}^{(k)}(\xe)  = 0, \qquad 
    \xe \in \set{S}_{e,1}^{\mathrm{c}}, \qquad 
    \liminf_{k \to \infty} \gamma_{\upe}^{(k)}(\xupe) = 0, \qquad 
    \xupe \in \set{S}_{\upe,1}^{\mathrm{c}}. \label{sec:algsin:eqn:129}
\end{align}
%----------------------------------------------------------------------------
Similar to the derivation of~\eqref{sec:algsin:eqn:110}, we have
%----------------------------------------------------------------------------
\begin{align}
    &\lim_{k \to \infty} \left. \pdv{}{ \gamma_{e}(\xe) }
    \log( \Zabsfn( (\vgam_{\psetpf} )^{1/\qf} ) )
    \right|_{ \vgam_{\psetpf} = \vgam_{\psetpf}^{(k)}  } 
    \nonumber\\
    &=
    \frac{1}{ \qe } \cdot
    \lim_{k \to \infty}
    \bigl( \gamma_{e}^{(k)}(\xe) \bigr)^{-(\qe-1)/\qe}
    \cdot \Biggl( 
    \frac{ \gamet^{(k+1)}(\xe) }{ \sum_{\xe} 
        \left( \gamma_{e}^{(k)}(\xe) \right)^{1/\qe} 
        \cdot \gamet^{(k+1)}(\xe) 
    }
    - \bigl( \gamma_{e}^{(k)}(\xe) \bigr)^{(\qe-1)/\qe} \Biggr)
    \nonumber\\
    &\overset{(a)}{=}   
    0,
    \qquad \xe \in \set{S}_{e,1}, \, e \in \setpf, \label{sec:algsin:eqn:128}
\end{align}
%----------------------------------------------------------------------------
where step $(a)$ follows from Lemma~\ref{sec:algsin:lem:4} with the substitution in~\eqref{sec:algsin:eqn:4} and the fact that because $ \liminf_{k \to \infty} \gamma_{e}^{(k)}(\xe) > 0 $ for $ \xe \in \set{S}_{e,1} $, there exists an $ \epsilon_{e,1} \in \sR_{>0} $ and an integer $ K \in \sZpp $ such that 
$ 0 < \bigl( \gamma_{e}^{(k)}(\xe) \bigr)^{-(\qe-1)/\qe} < \epsilon_{e,1} $ for all $ \xe \in \set{S}_{e,1} $ and $ k \geq K' $. For $ \upe \in \upsetpf $, we obtain the similar results:
%---------------------------------------------------------------------------
\begin{align}
    \lim_{k \to \infty} \left. \pdv{}{ \gamma_{\upe}(\xupe) }
    \log( \Zabsfn( (\vgam_{\psetpf} )^{1/\qf} ) )
    \right|_{ \vgam_{\psetpf} = \vgam_{\psetpf}^{(k)}  } 
    \cdot \gamma_{\upe}^{(k)}(\xupe) 
    &=  0, \qquad \xupe \in \setxupe, \label{sec:algsin:eqn:137}
    \\
    \lim_{k \to \infty} \left. \pdv{}{ \gamma_{\upe}(\xupe) }
    \log( \Zabsfn( (\vgam_{\psetpf} )^{1/\qf} ) )
    \right|_{ \vgam_{\psetpf} = \vgam_{\psetpf}^{(k)}  } 
    &=
    0,
    \qquad \xupe \in \set{S}_{\upe,1}. \label{sec:algsin:eqn:138}
\end{align}
%---------------------------------------------------------------------------
In the following derivations, we suppose that
%------------------------------------------------------------------------
\begin{align*}
    \limsup_{k_{1} \to \infty} 
    \left. \pdv{}{ \gamma_{e}(\xe) }
    \log( \Zabsfn( (\vgam_{\psetpf} )^{1/\qf} ) )
    \right|_{ \vgam_{\psetpf} = \vgam_{\psetpf}^{(k_{1})}  } 
    \cdot \gamma_{e}^{*}(\xe) \in \sR \cup \{ - \infty, + \infty \}, \qquad 
    \xe \in \set{S}_{e,2}, \, e \in \setpf, \nonumber\\
    \limsup_{k_{1} \to \infty} 
    \left. \pdv{}{ \gamma_{\upe}(\xupe) }
    \log( \Zabsfn( (\vgam_{\psetpf} )^{1/\qf} ) )
    \right|_{ \vgam_{\psetpf} = \vgam_{\psetpf}^{(k_{1})}  } 
    \cdot \gamma_{\upe}^{*}(\xupe) \in \sR \cup \{ - \infty, + \infty \}, \qquad 
    \xe \in \set{S}_{\upe,2}, \, \upe \in \upsetpf,
\end{align*}
%------------------------------------------------------------------------
where
%----------------------------------------------------------------------------
\begin{align}
    \set{S}_{e,2} & \defeq \left\{ 
        \xe \in \set{S}_{e,1}^{\mathrm{c}}
        \ \left| \ 
        \gamma_{e}^{*}(\xe) > 0
        % \limsup_{k_{1} \to \infty} 
        % \left. \pdv{}{ \gamma_{e}(\xe) }
        % \log( \Zabsfn( (\vgam_{\psetpf} )^{1/\qf} ) )
        % \right|_{ \vgam_{\psetpf} = \vgam_{\psetpf}^{(k_{1})}  } \neq 0
    \right. \right\}, \label{sec:algsin:eqn:113}\\
    \set{S}_{\upe,2} &\defeq \left\{ 
        \xupe \in \set{S}_{\upe,1}^{\mathrm{c}}
        \ \left| \ 
        \gamma_{\upe}^{*}(\xupe) > 0
        % \limsup_{k_{1} \to \infty} 
        % \left. \pdv{}{ \gamma_{\upe}(\xupe) }
        % \log( \Zabsfn( (\vgam_{\psetpf} )^{1/\qf} ) )
        % \right|_{ \vgam_{\psetpf} = \vgam_{\psetpf}^{(k_{1})}  } \neq 0
    \right. \right\}. \label{sec:algsin:eqn:136}
\end{align}
%----------------------------------------------------------------------------
Then the inequalities in~\eqref{sec:algsin:eqn:104} implies
%------------------------------------------------------------------------
\begin{align}
    &\log( \Zabsfn\Bigl( (\vgam_{\psetpf}^{*} )^{1/\qf} \Bigr) )
    \nonumber\\
    &\leq \liminf_{k \to \infty} 
    \Biggl( 
        \log( \Zabsfn\Bigl( (\vgam_{\psetpf}^{(k)} )^{1/\qf} \Bigr) )
        +
        \sum_{e \in \setpf}
        \sum_{\xe}
        \left. \pdv{}{ \gamma_{e}(\xe) }
        \log( \Zabsfn( (\vgam_{\psetpf} )^{1/\qf} ) )
        \right|_{ \vgam_{\psetpf} = \vgam_{\psetpf}^{(k)}  } 
        \cdot \Bigl( 
            \gamma_{e}^{*}(\xe) - \gamma_{e}^{(k)}(\xe) 
        \Bigr)
        \nonumber\\
        &\qquad\qquad+
        \sum_{\upe \in \upsetpf}
        \sum_{\xupe}
        \left. \pdv{}{ \gamma_{\upe}(\xupe) }
        \log( \Zabsfn( (\vgam_{\psetpf} )^{1/\qf} ) )
        \right|_{ \vgam_{\psetpf} = \vgam_{\psetpf}^{(k)}  } 
        \cdot \Bigl( 
            \gamma_{\upe}^{*}(\xupe) - \gamma_{\upe}^{(k)}(\xupe) 
        \Bigr)
    \Biggr)
    \nonumber\\
    &\overset{(a)}{=}
    \lim_{k \to \infty} 
    \log( \Zabsfn\Bigl( (\vgam_{\psetpf}^{(k)} )^{1/\qf} \Bigr) )
    + \liminf_{k \to \infty} 
    \Biggl( 
    \sum_{e \in \setpf}
    \sum_{\xe}
    \left. \pdv{}{ \gamma_{e}(\xe) }
    \log( \Zabsfn( (\vgam_{\psetpf} )^{1/\qf} ) )
    \right|_{ \vgam_{\psetpf} = \vgam_{\psetpf}^{(k)}  } 
    \cdot \Bigl( 
        \gamma_{e}^{*}(\xe) - \gamma_{e}^{(k)}(\xe) 
    \Bigr)
    \nonumber\\
    &\quad
    + \sum_{\upe \in \upsetpf}
    \sum_{\xupe}
    \left. \pdv{}{ \gamma_{\upe}(\xupe) }
    \log( \Zabsfn( (\vgam_{\psetpf} )^{1/\qf} ) )
    \right|_{ \vgam_{\psetpf} = \vgam_{\psetpf}^{(k)}  } 
    \cdot \Bigl( 
        \gamma_{\upe}^{*}(\xupe) - \gamma_{\upe}^{(k)}(\xupe) 
    \Bigr)
    \Biggr) 
    \nonumber\\
    &\overset{(b)}{\leq}
    \lim_{k \to \infty} 
    \log( \Zabsfn\Bigl( (\vgam_{\psetpf}^{(k)} )^{1/\qf} \Bigr) )
    + \liminf_{k \to \infty} 
    \Biggl(
        \sum_{e \in \setpf}
        \sum_{\xe \in \set{S}_{e,2}}
        \left. \pdv{}{ \gamma_{e}(\xe) }
        \log( \Zabsfn( (\vgam_{\psetpf} )^{1/\qf} ) )
        \right|_{ \vgam_{\psetpf} = \vgam_{\psetpf}^{(k)}  } 
        \cdot  \gamma_{e}^{*}(\xe)
        \nonumber\\
        & \quad 
        + \sum_{\upe \in \upsetpf}
        \sum_{\xupe \in \set{S}_{\upe,2}}
        \left. \pdv{}{ \gamma_{\upe}(\xupe) }
        \log( \Zabsfn( (\vgam_{\psetpf} )^{1/\qf} ) )
        \right|_{ \vgam_{\psetpf} = \vgam_{\psetpf}^{(k)}  } 
        \cdot  \gamma_{\upe}^{*}(\xupe)
    \Biggr) ,\label{sec:algsin:eqn:116}
\end{align}
%------------------------------------------------------------------------
where step $(a)$ follows from Lemma~\ref{sec:algsin:lem:8} with the substitution in~\eqref{sec:algsin:eqn:4},
and where step $(b)$ follows from the limits in~\eqref{sec:algsin:eqn:110},~\eqref{sec:algsin:eqn:128}--\eqref{sec:algsin:eqn:138}  and the definitions of $ \set{S}_{e,2} $ and $ \set{S}_{\upe,2} $ in~\eqref{sec:algsin:eqn:113} and~\eqref{sec:algsin:eqn:136}, respectively. By the definition of $ \vgam_{\psetpf}^{*} $ in Definition~\ref{sec:algsin:def:2} and the fact that $ \sum_{\xe} \gamma_{e}^{(k)}(\xe) =  \sum_{\xupe} \gamma_{\upe}^{(k)}(\xupe) = 1 $ for all $ \pe \in \psetpf $ and $ k \in \sZpp $ as defined in~\eqref{sec:algsin:eqn:89}, we have
%------------------------------------------------------------------------
\begin{align}
    \lim_{k \to \infty} 
    \log( \Zabsfn\Bigl( (\vgam_{\psetpf}^{(k)} )^{1/\qf} \Bigr) )
    \leq \log( \Zabsfn\Bigl( (\vgam_{\psetpf}^{*} )^{1/\qf} \Bigr) ),
    \label{sec:algsin:eqn:115}
\end{align}
%------------------------------------------------------------------------
which implies
%----------------------------------------------------------------------------
\begin{align}
    &
    \liminf_{k\to \infty} 
    \Biggl( 
    \sum_{e \in \setpf}
    \sum_{\xe \in \set{S}_{e,2}}
    \left. \pdv{}{ \gamma_{e}(\xe) }
    \log( \Zabsfn( (\vgam_{\psetpf} )^{1/\qf} ) )
    \right|_{ \vgam_{\psetpf} = \vgam_{\psetpf}^{(k)}  } 
    \cdot  \gamma_{e}^{*}(\xe)
    \nonumber\\
    &+ \sum_{\upe \in \upsetpf}
    \sum_{\xupe \in \set{S}_{\upe,2}}
    \left. \pdv{}{ \gamma_{\upe}(\xupe) }
    \log( \Zabsfn( (\vgam_{\psetpf} )^{1/\qf} ) )
    \right|_{ \vgam_{\psetpf} = \vgam_{\psetpf}^{(k)}  } 
    \cdot  \gamma_{\upe}^{*}(\xupe)
    \Biggr)
    \geq 0. \label{sec:algsin:eqn:127}
\end{align}
%----------------------------------------------------------------------------
Now we want to show that the limit inferior on the left-hand side of the inequality in~\eqref{sec:algsin:eqn:127} equals zero.
Because of the limits in~\eqref{sec:algsin:eqn:129} and the fact that $ \gamma_{e}^{(k)}(\xe) $ is positive and bounded for all $ \xe \in \setxe $, $ e \in \setpf $, and $ k \in \sZpp $, by the Bolzano–Weierstrass theorem~\cite[Theorem 3.4.8]{Bartle2010}, there exists a subsequence of $ \{ k \}_{k \in \sZpp} $, which is indexed by $ k_{1} \in \sZpp $, such that 
%----------------------------------------------------------------------------
\begin{align*}
    \lim_{k_{1} \to  \infty} \gamma_{e}^{(k_{1})}(\xe) 
    \in \sR_{\geq 0}, \quad 
    \lim_{k_{1} \to  \infty} \gamma_{\upe}^{(k_{1})}(\xupe) 
    \in \sR_{\geq 0}, \qquad 
    \pe = (\xe, \xupe) \in \set{S}_{e',1}^{\mathrm{c}} 
    \times \set{S}_{\upe,1}^{\mathrm{c}},\, 
    \pe = (e,\upe) \in \psetpf.
\end{align*}
%----------------------------------------------------------------------------
We define
%------------------------------------------------------------------------
\begin{align*}
    \set{S}_{e,3} & \defeq \left\{ 
        \xe \in \set{S}_{e,2}
        \ \left| \ 
        \lim_{k_{1} \to  \infty} \gamma_{e}^{(k_{1})}(\xe)
        = 0
    \right. \right\}, \\
    \set{S}_{\upe,3} &\defeq \left\{ 
        \xupe \in \set{S}_{\upe,2}
        \ \left| \ 
        \lim_{k_{1} \to  \infty} \gamma_{\upe}^{(k_{1})}(\xupe)
        = 0
        % \limsup_{k_{1} \to \infty} 
        % \left. \pdv{}{ \gamma_{\upe}(\xupe) }
        % \log( \Zabsfn( (\vgam_{\psetpf} )^{1/\qf} ) )
        % \right|_{ \vgam_{\psetpf} = \vgam_{\psetpf}^{(k_{1})}  } \neq 0
    \right. \right\}. 
\end{align*}
%------------------------------------------------------------------------
Because both $ \gamma_{e}^{(k_{1})}(\xe) $ and $ \gamma_{\upe}^{(k_{1})}(\xupe) $ are positive-valued for all $ \xe \in \set{S}_{e,2} $ and $ \xupe \in \set{S}_{\upe,2} $ and $ k_{1} \in \sZpp $, 
then there exists a subsequence of $ \{ k_{1} \}_{k_{1} \in \sZpp} $, which is indexed by $ k_{2} \in \sZpp $ such that
%----------------------------------------------------------------------------
\begin{align}
    \frac{ \gamma_{e}^{(k_{2}+1)}(\xe) }{ \gamma_{e}^{(k_{2})}(\xe) }
    <1, \qquad 
    \frac{ \gamma_{\upe}^{(k_{2}+1)}(\xupe) }{ \gamma_{\upe}^{(k_{2})}(\xupe) }
    < 1, \qquad \xpe = (\xe,\xupe) \in \set{S}_{e,3} \times \set{S}_{\upe,3}.
    \label{sec:algsin:eqn:135}
\end{align}
%----------------------------------------------------------------------------
Similar to the proof of~\eqref{sec:algsin:eqn:128}, we have
%----------------------------------------------------------------------------
\begin{align}
    &\liminf_{k_{2}\to \infty} 
    \Biggl( 
    \sum_{e \in \setpf}
    \sum_{\xe \in \set{S}_{e,2}}
    \left. \pdv{}{ \gamma_{e}(\xe) }
    \log( \Zabsfn( (\vgam_{\psetpf} )^{1/\qf} ) )
    \right|_{ \vgam_{\psetpf} = \vgam_{\psetpf}^{(k_{2})}  } 
    \!\!\!\!\!
    \cdot  \gamma_{e}^{*}(\xe)
    + \sum_{\upe \in \upsetpf}
    \sum_{\xupe \in \set{S}_{\upe,2}}
    \left. \pdv{}{ \gamma_{\upe}(\xupe) }
    \log( \Zabsfn( (\vgam_{\psetpf} )^{1/\qf} ) )
    \right|_{ \vgam_{\psetpf} = \vgam_{\psetpf}^{(k_{2})}  } 
    \!\!\!\!\!
    \cdot  \gamma_{\upe}^{*}(\xupe)
    \Biggr)
    \nonumber\\
    &= \liminf_{k_{2}\to \infty} 
    \Biggl( 
    \sum_{e \in \setpf}
    \sum_{\xe \in \set{S}_{e,3}}
    \left. \pdv{}{ \gamma_{e}(\xe) }
    \log( \Zabsfn( (\vgam_{\psetpf} )^{1/\qf} ) )
    \right|_{ \vgam_{\psetpf} = \vgam_{\psetpf}^{(k_{2})}  } 
    \!\!\!\!\!
    \cdot  \gamma_{e}^{*}(\xe)
    + \sum_{\upe \in \upsetpf}
    \sum_{\xupe \in \set{S}_{\upe,3}}
    \left. \pdv{}{ \gamma_{\upe}(\xupe) }
    \log( \Zabsfn( (\vgam_{\psetpf} )^{1/\qf} ) )
    \right|_{ \vgam_{\psetpf} = \vgam_{\psetpf}^{(k_{2})}  } 
    \!\!\!\!\!
    \cdot  \gamma_{\upe}^{*}(\xupe)
    \Biggr) 
    \label{sec:algsin:eqn:141}\\
    &\geq 0. \label{sec:algsin:eqn:140}
\end{align}
%----------------------------------------------------------------------------
We want to prove that the inequality in~\eqref{sec:algsin:eqn:140} is indeed an equality. We prove it by contradiction.
Suppose that the expression on the left-hand side of the inequality~\eqref{sec:algsin:eqn:140} is positive.
Because both $ \gamma_{e}^{*}(\xe) $ and $ \gamma_{\upe}^{*}(\xupe) $ are positive-valued for all $ \xe \in \set{S}_{e,2} $ and $ \xupe \in \set{S}_{\upe,2} $, the strict inequality in~\eqref{sec:algsin:eqn:140} implies
%------------------------------------------------------------------------
\begin{align}
    &\exists \xe' \in \set{S}_{e,3},\, \mathrm{s.t.}\ 
    \limsup_{k_{2} \to \infty} 
    \left. \pdv{}{ \gamma_{e}(\xe') }
    \log( \Zabsfn( (\vgam_{\psetpf} )^{1/\qf} ) )
    \right|_{ \vgam_{\psetpf} = \vgam_{\psetpf}^{(k_{2})}  } 
    > 0, 
    \label{sec:algsin:eqn:123}\\
    &\text{ or } \exists \xupe' \in \set{S}_{\upe,3},\,  \mathrm{s.t.}\
     \limsup_{k_{2} \to \infty} 
    \left. \pdv{}{ \gamma_{\upe}(\xupe') }
    \log( \Zabsfn( (\vgam_{\psetpf} )^{1/\qf} ) )
    \right|_{ \vgam_{\psetpf} = \vgam_{\psetpf}^{(k_{2})}  } > 0. 
    \label{sec:algsin:eqn:132}
\end{align}
%------------------------------------------------------------------------
%----------------------------------------------------------------------------
\begin{enumerate}
    \item We first consider~\eqref{sec:algsin:eqn:123}, which, by the expression of the partial derivatives in~\eqref{sec:algsin:eqn:108}, implies 
    %------------------------------------------------------------------------
    \begin{align*}
        &\limsup_{k_{2} \to \infty} 
        \bigl( \gamma_{e}^{(k_{2})}(\xe') \bigr)^{-(\qe-1)/\qe}
        \cdot 
        \frac{ \gamet^{(k_{2}+1)}(\xe') }{ \sum_{\xe} 
            ( \gamma_{e}^{(k_{2})}(\xe') )^{1/\qe} 
            \cdot \gamet^{(k_{2}+1)}(\xe') 
        }
        \nonumber\\
        &= \limsup_{k_{2} \to \infty} 
        \frac{ \gamet^{(k_{2}+1)}(\xe') }{ \| \gamet^{(k_{2}+1)}(\xe') \|_{ \qe/(\qe-1) } 
        \cdot 
        \bigl( \gamma_{e}^{(k_{2})}(\xe') \bigr)^{(\qe-1)/\qe} } 
        \cdot 
        \frac{ \| \gamet^{(k_{2}+1)}(\xe') \|_{ \qe/(\qe-1) }  
        }{ \sum_{\xe} 
            ( \gamma_{e}^{(k_{2})}(\xe') )^{1/\qe} 
            \cdot \gamet^{(k_{2}+1)}(\xe') 
        } 
        \nonumber\\
        &\overset{(a)}{=} \limsup_{k_{2} \to \infty} 
        \frac{ \left( \gamma_{e}^{(k_{2}+1)}(\xe') \right)^{(\qe-1)/\qe} 
        }{ \bigl( \gamma_{e}^{(k_{2})}(\xe') \bigr)^{(\qe-1)/\qe} }
        \cdot
        \frac{ 
                \Zabsfn\Bigl( (\vgam_{\psetpf}^{(k_{2}+1)} )^{1/\qe} \Bigr)
        }{  
            \Zabsfn\Bigl( (\vgam_{\psetpf}^{(k_{2})} )^{1/\qe} \Bigr)
        }\nonumber\\
        &\overset{(b)}{=} \limsup_{k_{2} \to \infty} 
        \frac{ \left( \gamma_{e}^{(k_{2}+1)}(\xe') \right)^{(\qe-1)/\qe} 
        }{ \bigl( \gamma_{e}^{(k_{2})}(\xe') \bigr)^{(\qe-1)/\qe} }
        \nonumber\\
        &> 1, \qquad \xe' \in \set{S}_{e,2},
    \end{align*}
    %------------------------------------------------------------------------
    where step $(a)$ follows from the expression of $ \gamma_{e}^{(k_{2}+1)}(\xe) $ in~\eqref{sec:algsin:eqn:89} and the equalities in~\eqref{sec:algsin:eqn:71}--\eqref{sec:algsin:eqn:92} with the substitution in~\eqref{sec:algsin:eqn:4}, 
    and where step $(b)$ follows from Lemma~\ref{sec:algsin:lem:8}, i.e., $ \lim_{k \to \infty} 
        \Zfnorm\Bigl( \vpsi_{\psetpf}^{(k)} \Bigr) $ exists and the fact that $ \Bigl\{ \Zfnorm\Bigl( \vpsi_{\psetpf}^{(k)} \Bigr) \Bigr\}_{ k \in \sZpp } $ is a monotonic sequence.
    For any $ \epsilon_{e} \in \sR_{>0} $ satisfying 
    %------------------------------------------------------------------------
    \begin{align*}
        \limsup_{k_{2} \to \infty} 
        \frac{ \left( \gamma_{e}^{(k_{2}+1)}(\xe') \right)^{(\qe-1)/\qe} 
        }{ \bigl( \gamma_{e}^{(k_{2})}(\xe') \bigr)^{(\qe-1)/\qe} } 
        > 1 +\epsilon_{e},
    \end{align*}
    %------------------------------------------------------------------------
    there exists a subsequence $ \{\gamma_{e}^{(k_{2})}(\xe')\}_{k_{2} \in \sZpp} $ of $ \{\gamma_{e}^{(k_{2})}(\xe')\}_{k_{2} \in \sZpp} $ such that
    %------------------------------------------------------------------------
    \begin{align*}
        \frac{ \left( \gamma_{e}^{(k_{2}+1)}(\xe') \right)^{(\qe-1)/\qe} 
        }{ \bigl( \gamma_{e}^{(k_{2})}(\xe') \bigr)^{(\qe-1)/\qe} } 
        > 1 +\epsilon_{e}, \qquad k_{2} \in \sZpp
    \end{align*}
    %------------------------------------------------------------------------
    which contradicts to~\eqref{sec:algsin:eqn:135}. Thus we have
    %------------------------------------------------------------------------
    \begin{align}
        &\limsup_{k_{2} \to \infty} 
        \left. \pdv{}{ \gamma_{e}(\xe') }
        \log( \Zabsfn( (\vgam_{\psetpf} )^{1/\qf} ) )
        \right|_{ \vgam_{\psetpf} = \vgam_{\psetpf}^{(k_{2})}  } 
        \cdot  \gamma_{e}^{*}(\xe') = 0. \label{sec:algsin:eqn:133}
    \end{align}
    %------------------------------------------------------------------------

    \item Similarly, by considering~\eqref{sec:algsin:eqn:132}, we also obtain contradictive statements, which proves
    %------------------------------------------------------------------------
    \begin{align}
        &\limsup_{k_{2} \to \infty} 
        \left. \pdv{}{ \gamma_{\upe}(\xupe') }
        \log( \Zabsfn( (\vgam_{\psetpf} )^{1/\qf} ) )
        \right|_{ \vgam_{\psetpf} = \vgam_{\psetpf}^{(k_{2})}  } 
        \cdot  \gamma_{\upe}^{*}(\xupe') = 0.
        \label{sec:algsin:eqn:134}
    \end{align}
    %------------------------------------------------------------------------
\end{enumerate}
%----------------------------------------------------------------------------
Combining the limit superior in~\eqref{sec:algsin:eqn:133} and~\eqref{sec:algsin:eqn:134} with the
inequalities~\eqref{sec:algsin:eqn:115} and~\eqref{sec:algsin:eqn:116}, we have
%------------------------------------------------------------------------
\begin{align}
    &\lim_{k_{2} \to \infty} 
    \left. \pdv{}{ \gamma_{e}(\xe) }
    \log( \Zabsfn( (\vgam_{\psetpf} )^{1/\qf} ) )
    \right|_{ \vgam_{\psetpf} = \vgam_{\psetpf}^{(k_{2})}  } 
    \cdot  \gamma_{e}^{*}(\xe) 
    =
    \lim_{k_{2} \to \infty} 
    \left. \pdv{}{ \gamma_{\upe}(\xupe) }
    \log( \Zabsfn( (\vgam_{\psetpf} )^{1/\qf} ) )
    \right|_{ \vgam_{\psetpf} = \vgam_{\psetpf}^{(k_{2})}  } 
    \cdot  \gamma_{\upe}^{*}(\xupe)
    = 0, \nonumber \\
    &\qquad \xpe = (\xe, \xupe) \in \set{S}_{e,3} \times 
    \set{S}_{\upe,3}, \, \pe \in \psetpf,
\end{align}
%------------------------------------------------------------------------
which by the equality in~\eqref{sec:algsin:eqn:141} implies the limit inferior on the left-hand side of the inequality in~\eqref{sec:algsin:eqn:127} equals zero and
%------------------------------------------------------------------------
\begin{align}
    &\log( \Zabsfn\Bigl( (\vgam_{\psetpf}^{*} )^{1/\qf} \Bigr) )
    =
    \lim_{k \to \infty} 
    \log( \Zabsfn\Bigl( (\vgam_{\psetpf}^{(k)} )^{1/\qf} \Bigr) ),
    \label{sec:algsin:eqn:118}\\
    &\log( \sig_{q}(|f|) )
    \overset{(a)}{=}
    \log( \Zabsfn\Bigl( (\vgam_{\psetpf}^{*} )^{1/\qf} \Bigr) )
    \overset{(b)}{=}
    \lim_{k \to \infty} 
    \log( \Zabsfn\Bigl( (\vgam_{\psetpf}^{(k)} )^{1/\qf} \Bigr) ),
    \nonumber
\end{align}
%------------------------------------------------------------------------
where step $(a)$ follows from Proposition~\ref{sec:algsin:prop:6}, 
and where step $(b)$ follows from~\eqref{sec:algsin:eqn:118}.
