# Supplementary material for: Finite-Graph-Cover-Based Analysis of Factor Graphs in Classical and Quantum Information Processing Systems
Source: arXiv:2412.05942 source file (2024-12-08)
Supplement: Supplementary file 6 [file props_tensor_norm_1.tex]

The absolute value of function $ Z_{\|f\|} $ defined in~\eqref{sec:algsin:eqn:32} can be written as
%-----------------------------------------------------------------------
\begin{align}
  \Bigl| Z_{\|f\|}(\vpsi_{\setpf},\vpsi_{\upsetpf}) \Bigr|
  &\overset{(a)}{=} 
  \Biggl| 
    \sum_{\ell_f \in \set{L}_f} 
    \lambda_{f}(\ell_f) \cdot 
    \Biggl( 
      \sum_{ \vx_{\setpf} }
      u_{f}(\vx_{\setpf},\ell_f) 
      \cdot \prod_{e \in \setpf} \psi_{e}(\xe) 
    \Biggr)
    \cdot \Biggl( 
      \sum_{ \vx_{\unpair{\setpf}} }
      \overline{u_{f}(\vx_{\unpair{\setpf}},\ell_f)}
      \cdot \prod_{e \in \setpf} \psi_{\upe}(\xupe) 
    \Biggr) 
  \Biggr|
  \nonumber\\
  &\overset{(b)}{\leq} 
  \sum_{\ell_f \in \set{L}_f} 
  \lambda_{f}(\ell_f) \cdot 
  \Biggl| 
    \sum_{ \vx_{\setpf} }
    u_{f}(\vx_{\setpf},\ell_f) 
    \cdot \prod_{e \in \setpf} \psi_{e}(\xe) 
  \Biggr|
  \cdot \Biggl| 
    \sum_{ \vx_{\unpair{\setpf}} }
    \overline{u_{f}(\vx_{\unpair{\setpf}},\ell_f)}
    \cdot \prod_{e \in \setpf} \psi_{\upe}(\xupe) 
  \Biggr|
  \nonumber\\
  &\overset{(c)}{\leq} 
  \max\Biggl(
    \sum_{\ell_f \in \set{L}_f} 
    \lambda_{f}(\ell_f) \cdot 
    \Biggl| 
      \sum_{ \vx_{\setpf} }
      u_{f}(\vx_{\setpf},\ell_f) 
      \cdot \prod_{e \in \setpf} \psi_{e}(\xe) 
    \Biggr|
    \cdot \Biggl| 
      \sum_{ \vx_{\unpair{\setpf}} }
      \overline{u_{f}(\vx_{\unpair{\setpf}},\ell_f)}
      \cdot \prod_{e \in \setpf} \psi_{e}(\xupe) 
    \Biggr|
    ,\nonumber\\
    &\quad \sum_{\ell_f \in \set{L}_f} 
    \lambda_{f}(\ell_f) \cdot 
    \Biggl| 
      \sum_{ \vx_{\setpf} }
      u_{f}(\vx_{\setpf},\ell_f) 
      \cdot \prod_{\pe \in \setpf} \psi_{\upe}(\xe) 
    \Biggr|
    \cdot \Biggl| 
      \sum_{ \vx_{\unpair{\setpf}} }
      \overline{u_{f}(\vx_{\unpair{\setpf}},\ell_f)}
      \cdot \prod_{e \in \setpf} \psi_{\upe}(\xupe) 
    \Biggr|
  \Biggr) 
  \label{sec:algsin:eqn:73}\\
  &\in \sR_{\geq 0}, \nonumber
\end{align}
%-----------------------------------------------------------------------}
where step $(a)$ follows from the fact that for a strict-sense PE-NFG $ N $, each local function $ f \in \setF $ has a decomposition as shown in~\eqref{sec:DENFG:eqn:5},
where step $(b)$ follows from the triangular inequality and
$ \lambda_{f}(\ell_f) \in \sR_{\geq 0} $ for all $ \ell_f $ in $ \set{L}_f $ as shown in~\eqref{sec:DENFG:eqn:8}, 
and where step $(c)$ follows from the Cauchy-Schwarz inequality.
By setting $ \vpsi_{\upsetpf} = \overline{ \vpsi_{\setpf} } $, we have
%-----------------------------------------------------------------------
\begin{align}
  Z_{\|f\|}(\vpsi_{\setpf},\overline{\vpsi_{\setpf}})
  &\overset{(a)}{=} \sum_{\ell_f \in \set{L}_f} 
    \lambda_{f}(\ell_f) \cdot 
    \Biggl( 
      \sum_{ \vx_{\setpf} }
      u_{f}(\vx_{\setpf},\ell_f) 
      \cdot \prod_{e \in \setpf} \psi_{e}(\xe) 
    \Biggr)
    \cdot \Biggl( 
      \sum_{ \vx_{\unpair{\setpf}} }
      \overline{u_{f}(\vx_{\unpair{\setpf}},\ell_f)
      \cdot \prod_{e \in \setpf} \psi_{e}(\xupe) }
    \Biggr) 
  \nonumber\\
  &= \sum_{\ell_f \in \set{L}_f} 
    \lambda_{f}(\ell_f) \cdot 
    \Biggl| 
      \sum_{ \vx_{\setpf} }
      u_{f}(\vx_{\setpf},\ell_f) 
      \cdot \prod_{e \in \setpf} \psi_{e}(\xe) 
    \Biggr|
    \cdot \Biggl| 
      \sum_{ \vx_{\unpair{\setpf}} }
      u_{f}(\vx_{\unpair{\setpf}},\ell_f)
      \cdot \prod_{e \in \setpf} \psi_{e}(\xupe)
    \Biggr|
  \label{sec:algsin:eqn:74}\\
  &\overset{(b)}{\in} \sR_{\geq 0}. \nonumber
\end{align}
%-----------------------------------------------------------------------
where step $(a)$ follows from the fact that for a strict-sense PE-NFG $ N $, each local function $ f \in \setF $ has a decomposition as shown in~\eqref{sec:DENFG:eqn:5}, and
where step $(b)$ follows from $ \lambda_{f}(\ell_f) \in \sR_{\geq 0} $ for all $ \ell_f $ in $ \set{L}_f $ as shown in~\eqref{sec:DENFG:eqn:8}. Combining~\eqref{sec:algsin:eqn:74} with the inequality in~\eqref{sec:algsin:eqn:73}, we know that it is sufficient to solve the optimization problem in~\eqref{sec:algsin:eqn:28} for solving $ \sig_{q}(f) $.
