# Supplementary material for: Finite-Graph-Cover-Based Analysis of Factor Graphs in Classical and Quantum Information Processing Systems
Source: arXiv:2412.05942 source file (2024-12-08)
Supplement: Supplementary file 8 [file the_message_conjugate_penfg.tex]

It is sufficient to consider the case where $t = 1$. The proof for $t \in \sZ_{\geq 2}$ is similar and is thus omitted.

For $ t =1 $, considering a pair of edge $ \pe \in \psetEfull $ connecting function nodes $ f_{i} $ and $ f_{j} $, we have
%------------------------------------------------------------------------
\begin{align*}
  \overline{\mu_{\upefi}^{(1)}(\zupe)}
  &= \overline{ \bigl( \kappa_{\upefi}^{(1)} \bigr)^{\!-1} } 
    \cdot
        \sum_{\vx_{\psetpfj}: \, \xupe = \zupe}
        \overline{ f_{j}\bigl( \vx_{\psetpfj} \bigr) }
        \cdot
        \overline{ \mu_{\efj}^{(0)}(\xe) }
        \cdot
        \prod_{\pe'\in \psetpfj \setminus \pe}
        \overline{ \mu_{\epfj}^{(0)}(x_{e'}) }
        \cdot 
        \overline{ \mu_{\upepfj}^{(0)}(x_{\upe'}) }
    \nonumber\\
    &\overset{(a)}{=}
    \overline{ \bigl( \kappa_{\upefi}^{(1)} \bigr)^{\!-1} } 
    \cdot
    \sum_{\vx_{\psetpfj}: \, \xupe = \zupe}
    f_{j}(\vx_{\upsetpfj},\vx_{\setpfj})
    \cdot
    \overline{ \mu_{\efj}^{(0)}(\xe)}
    \cdot
    \prod_{\pe'\in \psetpfj \setminus \pe}
    \overline{ \mu_{\epfj}^{(0)}(x_{e'}) }
    \cdot 
    \overline{ \mu_{\upepfj}^{(0)}(x_{\upe'}) }
    \nonumber\\
    &\overset{(b)}{=}
    \overline{ \bigl( \kappa_{\upefi}^{(1)} \bigr)^{\!-1} } 
    \cdot
    \sum_{\vx_{\psetpfj}: \, \xupe = \zupe}
    f_{j}(\vx_{\upsetpfj},\vx_{\setpfj})
    \cdot
    \mu_{\upefj}^{(0)}(\xe)
    \cdot
    \prod_{\pe'\in \psetpfj \setminus \pe}
    \mu_{\upepfj}^{(0)}(x_{e'})
    \cdot 
    \mu_{\epfj}^{(0)}(x_{\upe'})
    \nonumber\\
    &\overset{(c)}{=}
    \overline{ \bigl( \kappa_{\upefi}^{(1)} \bigr)^{\!-1} } 
    \cdot
    \underbrace{
    \sum_{\vx_{\psetpfj}: \, \xe = \zupe }
    f_{j}(\vx_{\setpfj},\vx_{\upsetpfj})
    \cdot
    \mu_{\upefj}^{(0)}(\xupe)
    \cdot
    \prod_{\pe'\in \psetpfj \setminus \pe}
    \mu_{\upepfj}^{(0)}(x_{\upe'})
    \cdot 
    \mu_{\epfj}^{(0)}(x_{e'})
    }_{ \overset{(d)}{=} \kappa_{\efi}^{(1)} \cdot \mu_{\efi}^{(1)}(\zupe) }
    \nonumber\\
    &\overset{(e)}{=}
    \mu_{\efi}^{(1)}(\zupe), \qquad \ze \in \setxe,\, 
    e=(f_{i}, f_{j}) \in \setEfull,\, \upe=(f_{i}, f_{j}) \in \upsetEfull,
\end{align*}
%------------------------------------------------------------------------
where step $(a)$ follows from the fact that the Choi matrix $ \matr{C}_{f_{j}} $ is a PSD matrix:
%--------------------------------------------------------------------
\begin{align*}
    \overline{ f_{j}( \vx_{\psetpfj} ) } = 
    \overline{ f_{j}( \vx_{\setpfj}, \vx_{\upsetpfj} ) }
    = f_{j}( \vx_{\upsetpfj}, \vx_{\setpfj} ),
\end{align*}
%--------------------------------------------------------------------
where step $(b)$ follows from Item~\ref{sec:DENFG:def:4:item:1} in Definition~\ref{sec:DENFG:def:4}: $ \setxe = \setxupe $ for all $ \pe \in \setEfull $, and the initialization of the messages in step 1 in Definition~\ref{sec:DENFG:def:2}:
%--------------------------------------------------------------------
\begin{align*}
    \mu_{\upef}^{(0)}(\xe) = \overline{ \mu_{\ef}^{(0)}(\xe) },
    \qquad \xe \in \setxe,\, e \in \setpf, \, f \in \setF,
\end{align*}
%--------------------------------------------------------------------
where step $(c)$ follows from the fact that because of $ \setxe = \setxupe $ for all $ \pe \in \setEfull $, switching $ \xe $ and $ \xupe $ keeps the expression on the right-hand side unchanged,
where step $(d)$ follows from the update rule of $ \mu_{\efi}^{(1)} $ in~\eqref{sec:DENFG:eqn:10},
and where step $(e)$ follows from the following facts:
%---------------------------------------------------------------------------
\begin{itemize}
  \item from step $(d)$, the message $ \overline{\mu_{\upefi}^{(1)}(\zupe)} $ is proportional to $ \mu_{\efi}^{(1)}(\zupe) $;

  \item both the messages $ \mu_{\efi}^{(1)} $ and $ \mu_{\upefi}^{(1)} $ are normalized: 
  %-------------------------------------------------------------------
  \begin{align*}
    \sum_{x_{e}} \mu_{\efi}^{(t)}(x_{e})
    = \sum_{x_{\upe}} \mu_{\upefi}^{(t)}(x_{\upe}) 
    = 1.
  \end{align*}
  %-------------------------------------------------------------------
\end{itemize}
%---------------------------------------------------------------------------
